# Supplementary material for: High-$T_{\rm c}$ Ag$_x$BC and Cu$_x$BC superconductors accessible via topochemical reactions
Source: arXiv:2507.14281 source file (2025-07-23)
Supplement: Supplementary file 1 [file supplemental.pdf]

# Supplemental Material: High-$T_c$ $Ag_xBC$ and $Cu_xBC$ superconductors accessible via topochemical reactions

Daviti Gochitashvili,[1] Charlsey R. Tomassetti,[1] Elena R. Margine,[1] and Aleksey N. Kolmogorov[1,*]

[1] *Department of Physics, Applied Physics, and Astronomy, Binghamton University-SUNY, Binghamton, New York 13902, USA*

(Dated: July 17, 2025)

* kolmogorov@binghamton.edu

| | | |
|---|---|---|
| I | Table I Topochemical reaction energies for NaBC precursor | 3 |
| II | Figure 1 Distance to convex hull as function of $T$ for Na-B-C and Li-Na-B-C | 3 |
| III | Figure 2 Phonon dispersion of mP6-CuBC and hP3-CuBC | 4 |
| IV | Figure 3 AIMD simulation of hP3-AgBC | 4 |
| V | Figure 4 Crystal structures of two $AgGaO_2$ polymorphs | 5 |
| VI | Figure 5 Relative stabilities of quaternary $Li_{x-y}M_yBC$ compounds (M = Cu or Ag) | 6 |
| VII | Figure 6 Electronic properties of hP3-CuBC and hP3-AgBC | 7 |
| VIII | Figure 7 Pressure dependence of $\omega_A$ in hP3-CuBC and hP3-CuBC | 7 |
| IX | Figure 8 Dependence of isotropic Midgal-Eliashberg $T_c$ with BC-$p_{x,y}$ DOS contribution | 8 |
| X | Figure 9 Phonon dispersions and $\alpha^2F(\omega)$ of Li-Cu-BC and Li-Ag-BC phases | 9 |
| XI | Figure 10 Band structure of AgBC with atoms displaced along phonon eigenvectors | 10 |
| XII | Figure 11 Phonon dispersion of AgBC with branches broadened by $\lambda_{\mathbf{k}\nu}$ | 10 |
| XIII | Figure 12 Anisotropic superconducting gap of AgBC with doping | 10 |
| XIV | Note I - Energy units conversion | 11 |
| XV | Note II - Approximation of the configurational free energy in $Li_{1-y}M_yBC$ (M = Cu or Ag) | 12 |
| XVI | Table II - Structures used in topochemical reactions | 13 |
| XVII | Table III - Summary of computational settings for superconductivity screening | 14 |
| XVIII | Listing 1-40 - Structural information for select phases in CIF format | 15 |
| XIX | Bibliography | 35 |

TABLE I. Calculated topochemical reaction energies in kJ per mole for the theoretical NaBC precursor and different ion sources.

| Precursor compound | Derived compound | $\Delta E_{\rm react}$ (kJ/mol) M | MI | MBr | MCl | $MNO_3$ |
|---|---|---|---|---|---|---|
| NaBC | CuBC | +58 | −173 | −215 | −232 | |
| NaBC | AgBC | +97 | −122 | −159 | −184 | −19 |

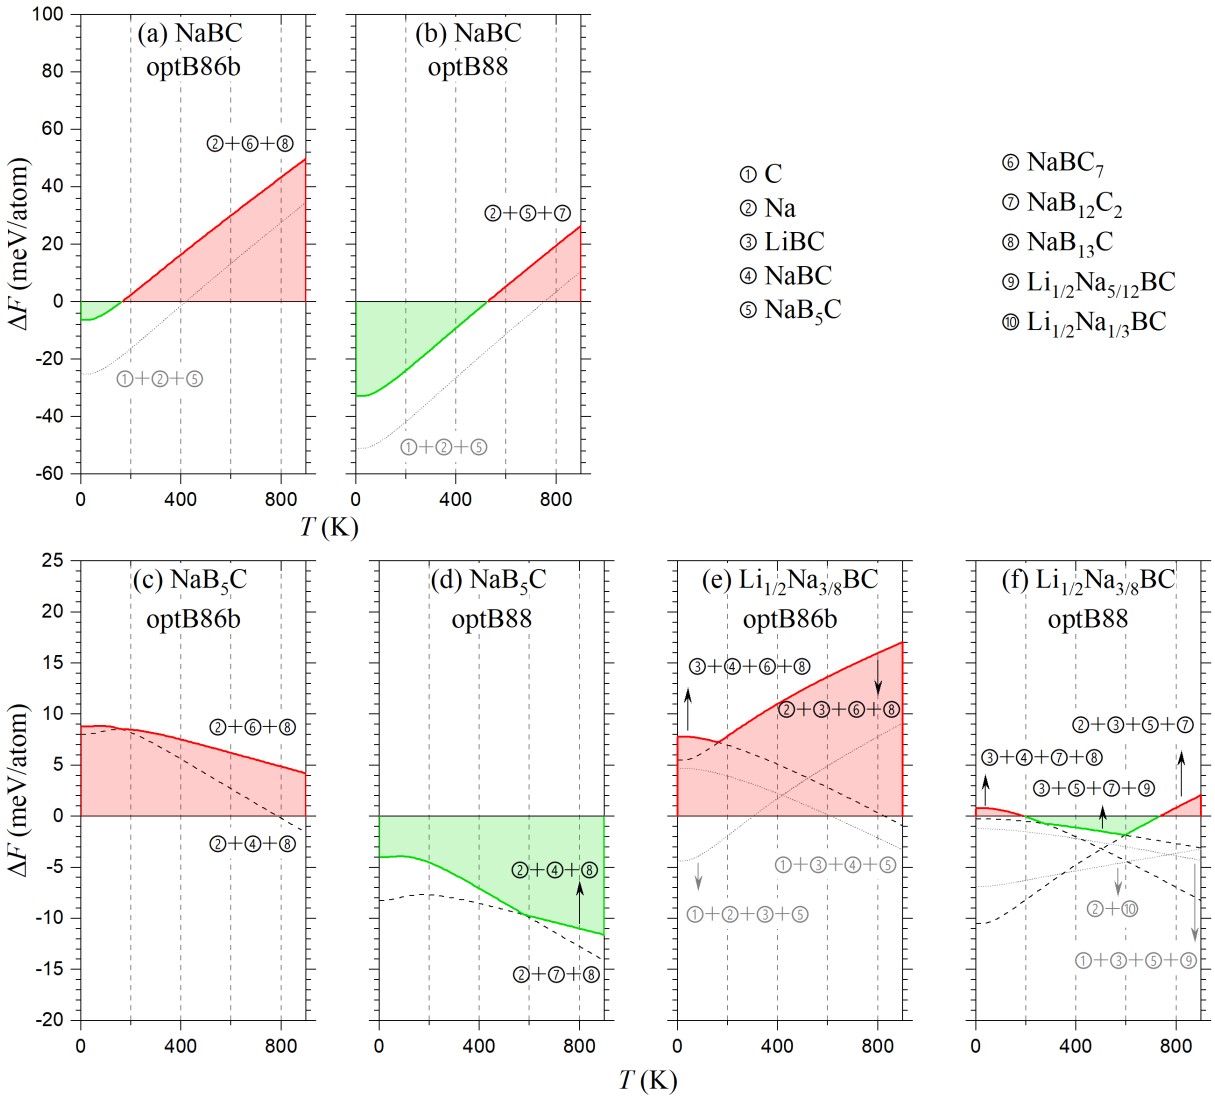


FIG. 1. Distance to the convex hull as a function of temperature for NaBC, $NaB_5C$, and a proposed Li–Na borocarbide. Details on the theoretical mP35-$Li_{1/2}Na_{5/12}BC$, mP23-$Li_{1/2}Na_{3/8}BC$, and mP34-$Li_{1/2}Na_{1/3}BC$ phases can be found in Ref. [1]. Different lines correspond to the lowest-free energy combinations among all observed ground states or previously proposed phases (circled numbers). With the addition of the $NaBC_7$ and $NaB_{12}C_2$ phases, NaBC appears below the known convex hull at lower temperatures than previously predicted in Ref. [1] (under 170 K for the optB86b-vdW and 520 K for the optB88-vdW functionals). Notably, the constructed ordered oP14 model of the $NaB_5C$ disordered compound becomes destabilized in the opB86b-vdW approximation with respect to mixtures of Na, $NaBC_7$, and $NaB_{13}C$, and Na, NaBC, and $NaB_{13}C$.

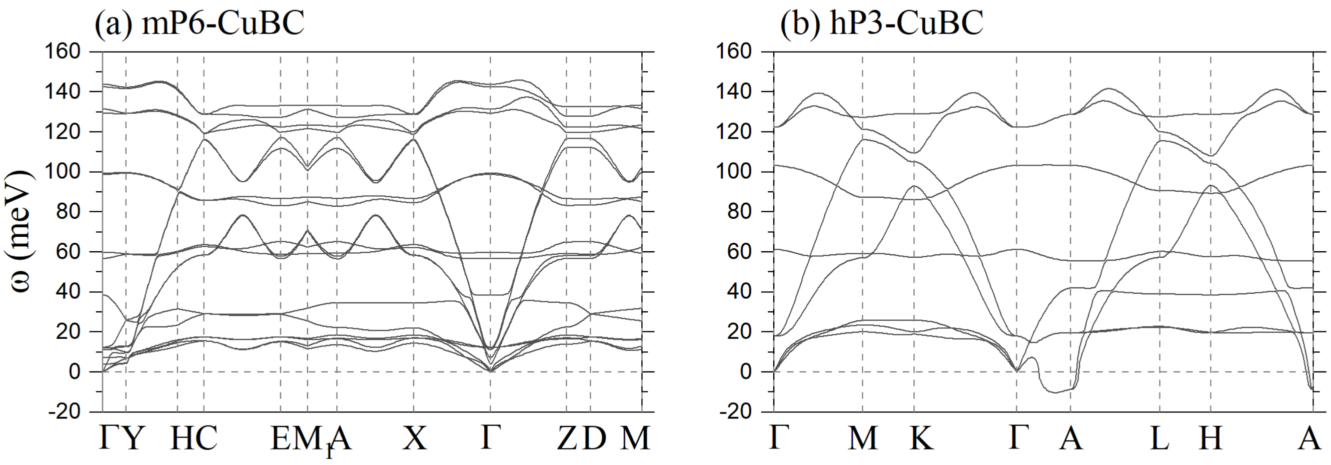


FIG. 2. Phonon dispersions calculated with QUANTUM ESPRESSO for (a) mP6-CuBC and (b) hP3-CuBC. The dynamical instability of hP3-CuBC is resolved via shearing of the BC layers that generates the mP6 structure with tilted C-Cu-C dumbbells.

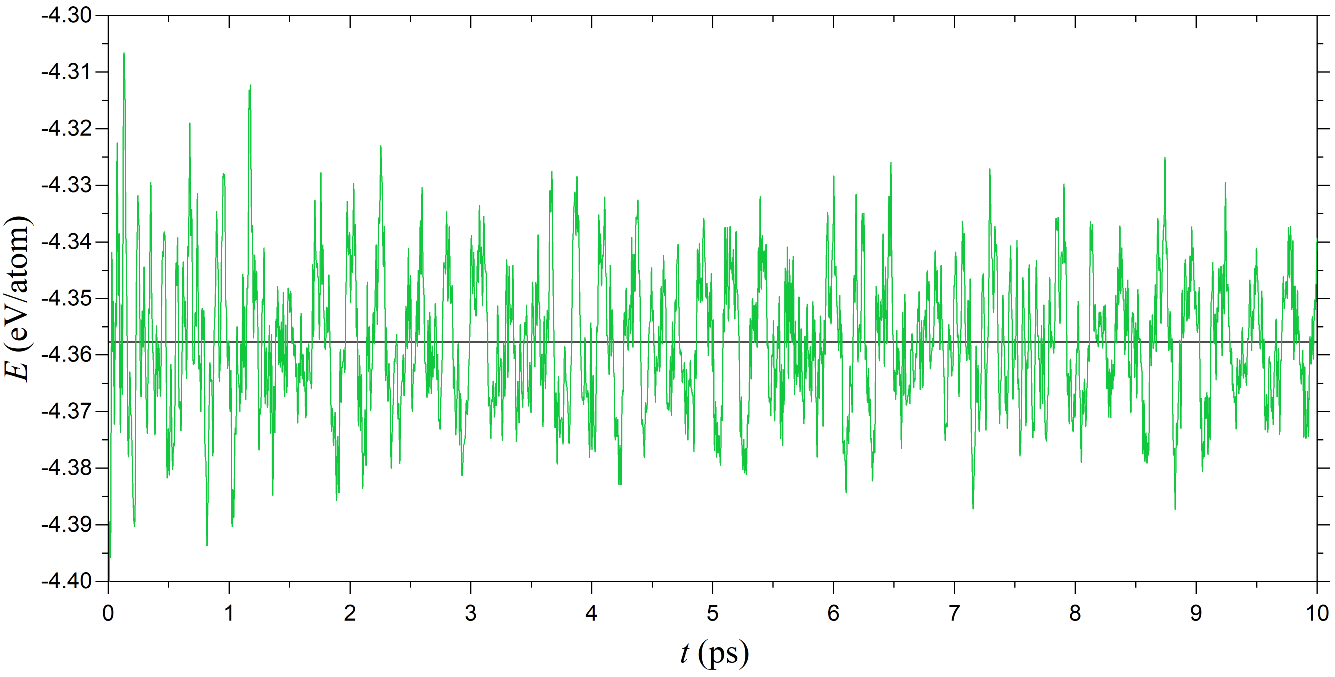


FIG. 3. Energy profile during AIMD NVT simulation at 600 K performed with VASP for the $3 \times 3 \times 2$ supercell of hP3-AgBC, indicating the absence of competing low-energy configurations. To confirm that the system remained in the original basin, we selected and examined 20 snapshots along the trajectory. The most visible deviation from the original structure involved moderate interlayer shifts, expected because of the particular flatness of the potential energy surface along directions corresponding to sheer of BC layers. Nevertheless, all considered structures maintained the connectivity of honeycomb BC layers and relaxed back to the starting hP3 configuration upon local re-optimization.

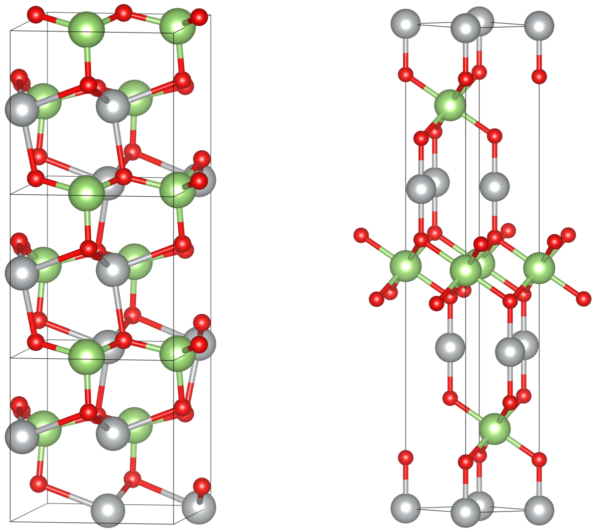

(a) oP16-$AgGaO_2$ ($Pna2_1$) (b) hR12-$AgGaO_2$ ($R\bar{3}m$)

FIG. 4. Crystal structures of two $AgGaO_2$ polymorphs. (a) The wurtzite oP16-$AgGaO_2$ phase synthesized via topotactic reactions by Suzuki et al. [2]. (b) hR12-$AgGaO_2$ phase identified in our global structure search. The rhombohedral polymorph with O–Ag–O dumbbells, 0.123 eV/atom below the reported orthorhombic counterpart, was found within 4 generations of a 20-member population in the $Ag_2Ga_2O_4$ evolutionary search starting from random configurations. A similar run for $Cu_2Ga_2O_4$ converged to the same rhombohedral structure, 0.179 eV/atom below the wurtzite type, within 10 generations. The global searches were not exhaustive and only served to illustrate the metastability of the materials synthesized via topotectic ion exchange.

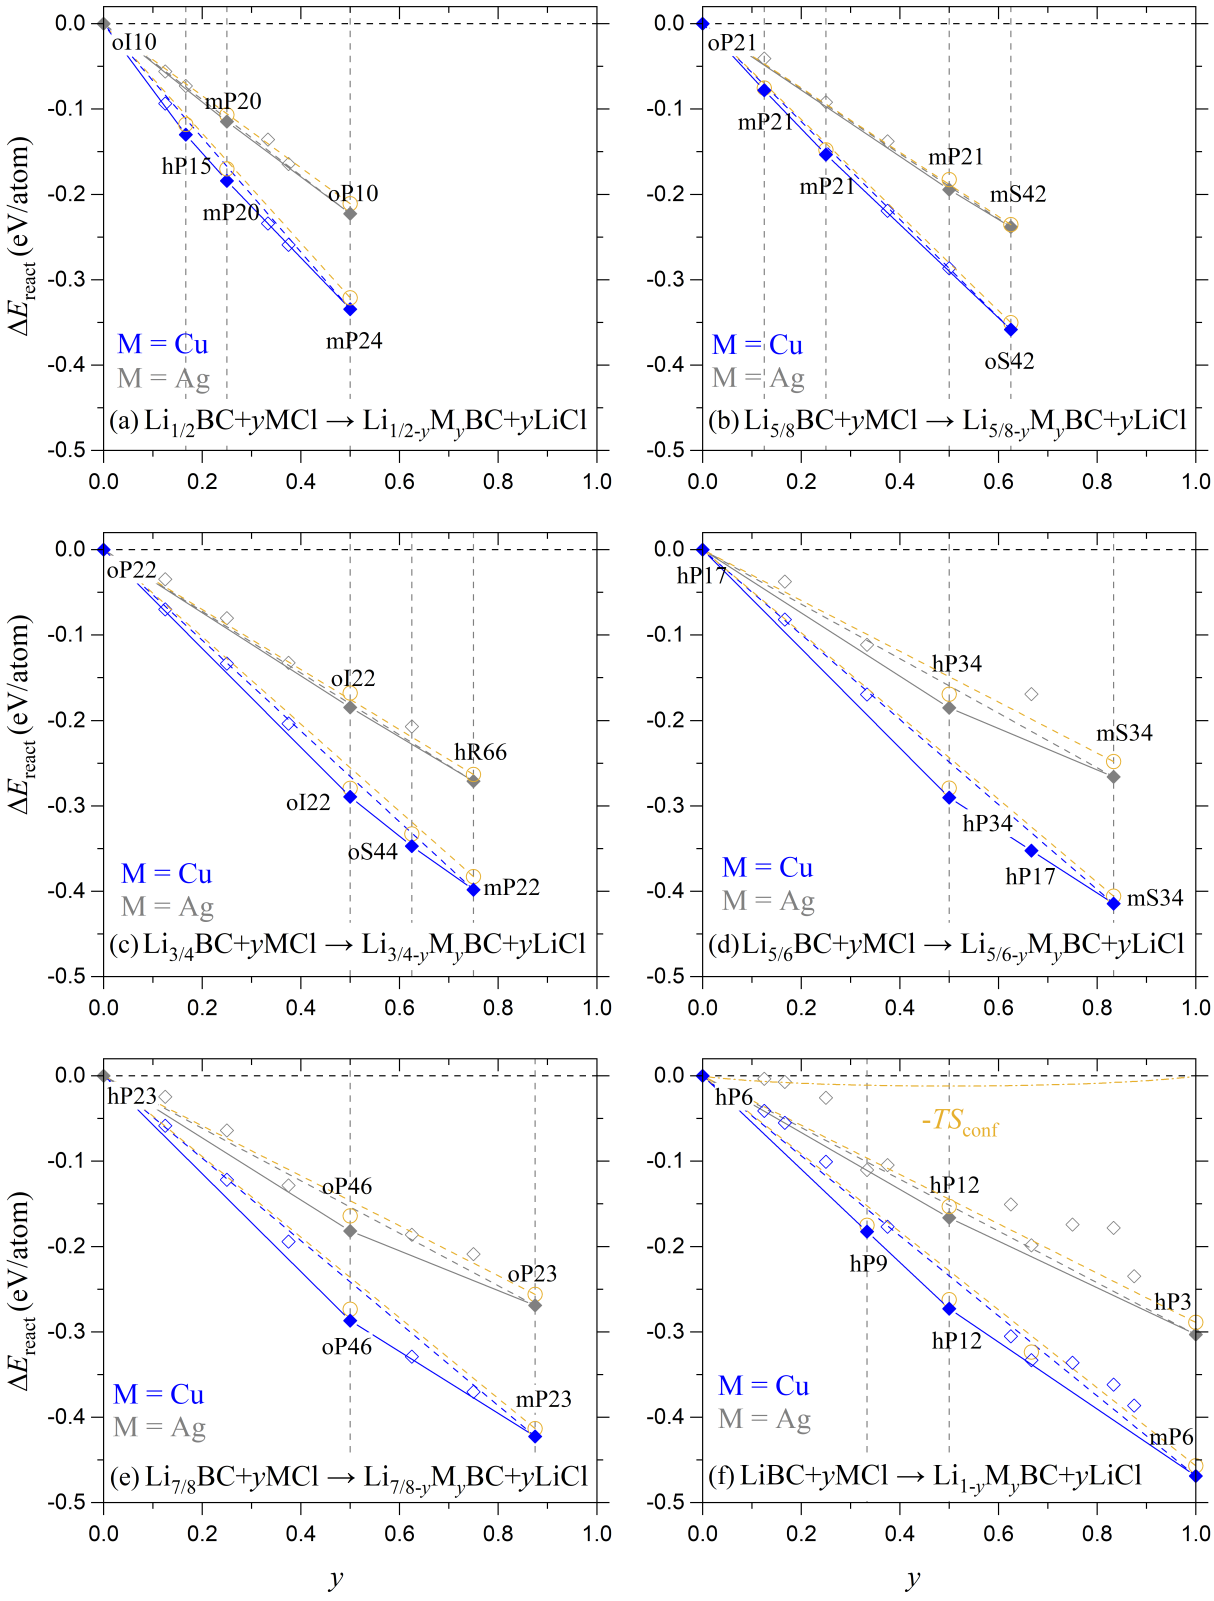


FIG. 5. Free energy per atom of topochemical reactions between $Li_xBC$ and $y$MCl forming $Li_xM_{x-y}BC$ and $y$LiCl (M = Cu or Ag) for $x$ equal to (a) 1/2, (b) 5/8, (c) 3/4, (d) 5/6, (e) 7/8, and (f) 1. Blue and gray colors denote data at 0 K, while yellow color corresponds to data at 600 K. The (hollow) solid points mark quaternary phases (meta)stable with respect to $Li_xBC$ and $M_xBC$. The dash-dot line in panel (f) accounts for the $S_{conf}$ contribution.

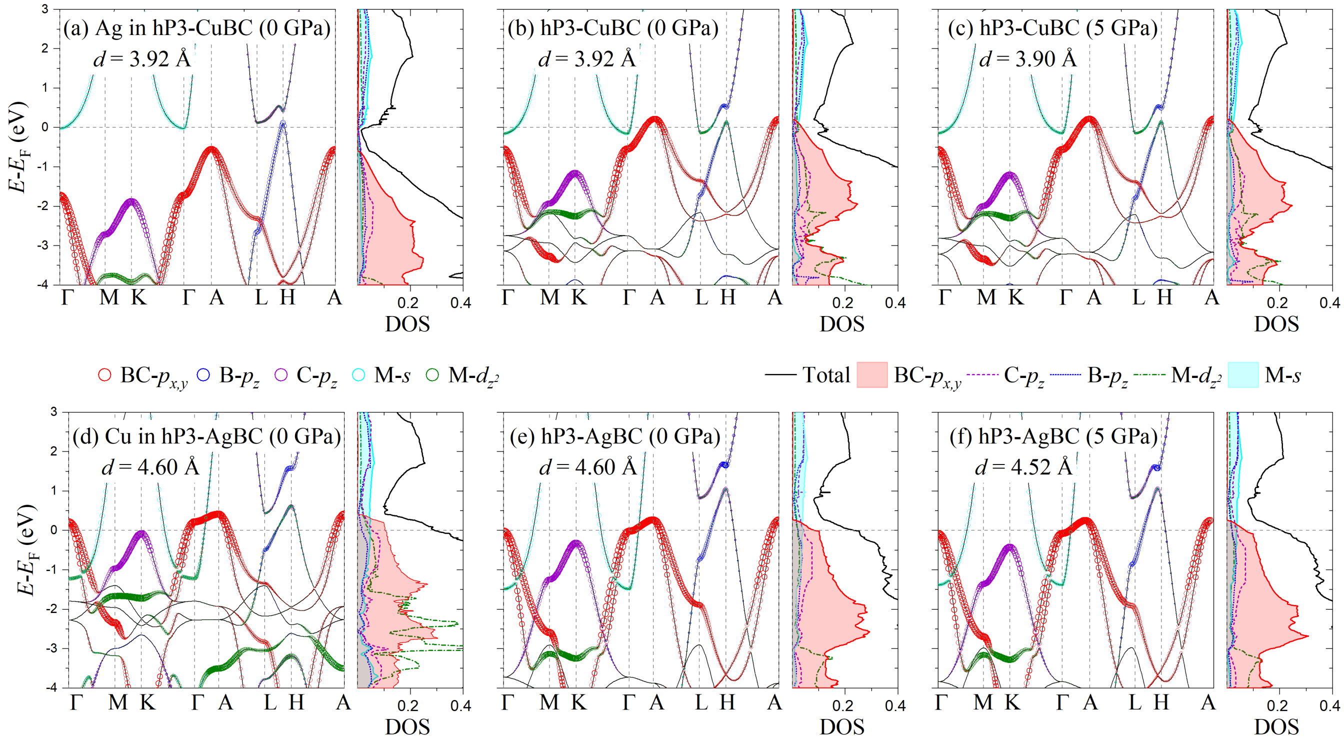


FIG. 6. Orbital-resolved electronic band structure and DOS in states/(eV atom) in hP3-CuBC and hP3-AgBC phases. The $p_{x,y}$ characters of B and C are combined, and only the $d_{z^2}$ character of the $d$ states is shown for Cu or Ag. To illustrate the effect of the interlayer spacing $d$ on the electronic structure, we display the results for structures under different conditions: (b,e) optimized at 0 GPa; (c,f) optimized at 5 GPa; and (a,d) optimized at 0 GPa and kept fixed while Cu is swapped for Ag and vice versa. The compression leads to negligible electronic structure responses. The Ag-to-Cu exchange in (d) raises the $s$ band edge by 0.3 eV at Γ and further hole-dopes the BC-$p_{x,y}$ states, which now cross the Fermi level between Γ and K and generate Fermi surface cylinders along Γ-A. The Cu-to-Ag exchange in (a) shifts the BC-$p_{x,y}$ states below the Fermi level. Overall, the steric effects are relatively moderate compared to the substantial rearrangements of the metal-$s$ and BC-$p_{x,y}$ states driven by changes in the interlayer spacing, which is ultimately controlled by the metal ion size.

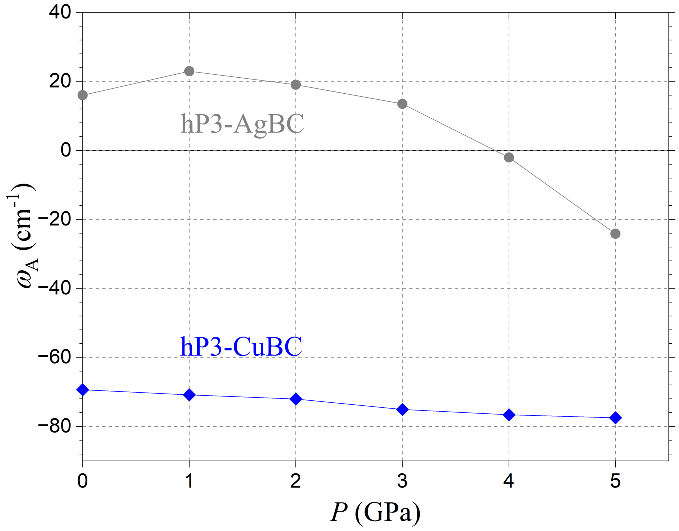


FIG. 7. Pressure dependence of the phonon mode shearing BC layers in the hP3-CuBC and hP3-AgBC phases. The linear response calculations were performed with VASP for unit cells doubled along the $c$ axis. The hP3-AgBC becomes dynamically unstable above 4 GPa.

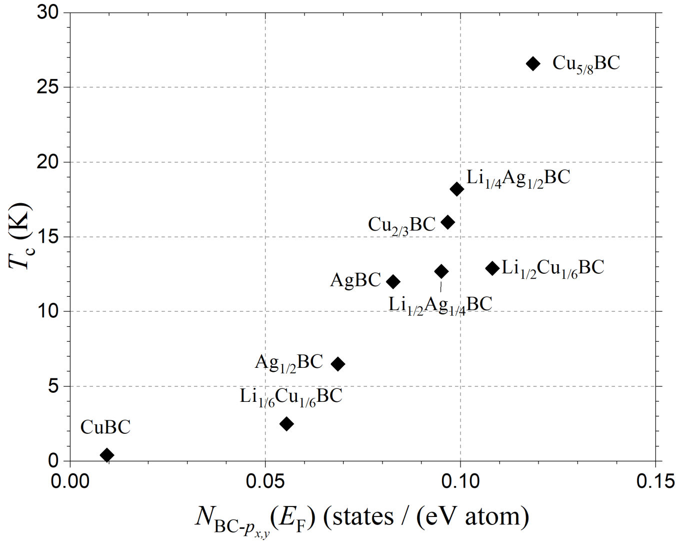


FIG. 8. Isotropic Migdal-Eliashberg critical temperatures as a function of the projected DOS from BC-$p_{x,y}$ (states/(eV atom)). The Eliashberg spectral functions were calculated on coarse grids within the PHonon code of QUANTUM ESPRESSO. Without interpolation to fine **k**- and **q**-grids, the estimates display only the general trend of $T_c$. Taking into account anisotropy is expected to enhance the critical temperatures, potentially fivefold (see Fig. 7).

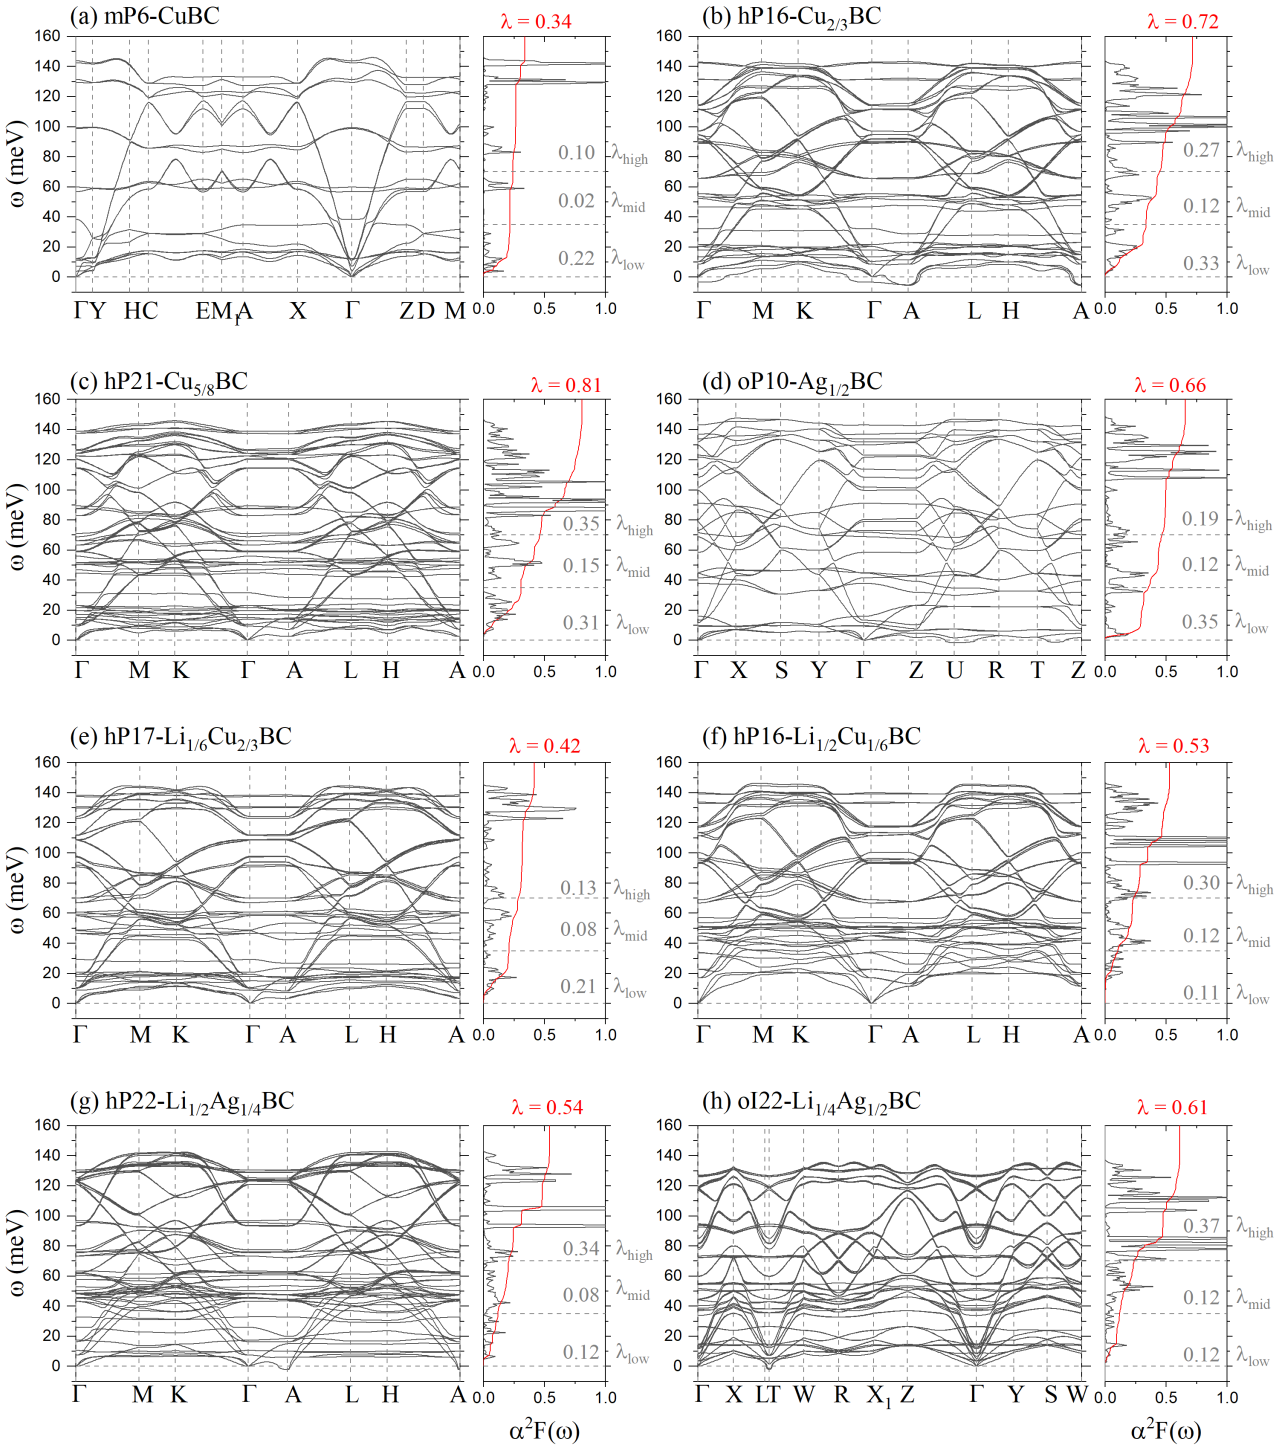


FIG. 9. Phonon dispersions and Eliashberg spectral functions of select phases screened for appreciable electron-phonon (e-ph) coupling with Quantum ESPRESSO. The e-ph coupling contributed by frequencies below 35 meV ($\lambda_{\mathrm{low}}$), between 35 and 70 meV ($\lambda_{\mathrm{mid}}$), and above 70 meV ($\lambda_{\mathrm{high}}$) are denoted in gray, summing to the total e-ph coupling $\lambda$, shown in red.

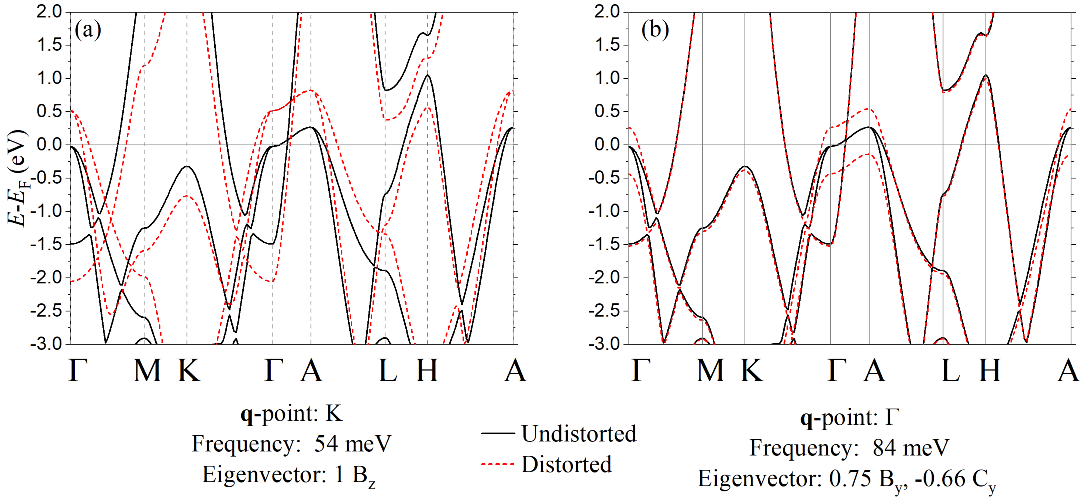


FIG. 10. Band structure of AgBC calculated with QUANTUM ESPRESSO in the hP3 structure (solid black lines) and structures with atoms displaced along specific normalized phonon eigenvectors using (a) 0.5 Å and (b) 0.02 Å scaling factors (dashed red lines). (a) The distortion corresponding to the K-point eigenmode that displaces B atoms along $z$ causes equally large responses of all three Ag-$s$, BC-$p_{x,y}$, and BC-$p_z$ bands crossing the Fermi level. (b) The distortion corresponding to the Γ-point in-plane BC bond stretching eigenmode results in predominant splitting of only the BC-$p_{x,y}$ band.

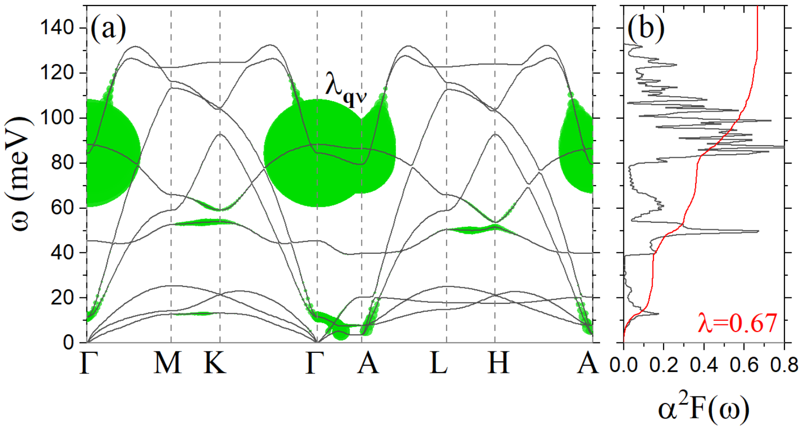


FIG. 11. Phonon dispersion and Eliashberg spectral function of hP3-AgBC, where the phonon branches are broadened by the e-ph coupling strength $\lambda_{\mathbf{q}\nu}$, showcasing the modes and high-symmetry directions that have the strongest contributions to pairing.

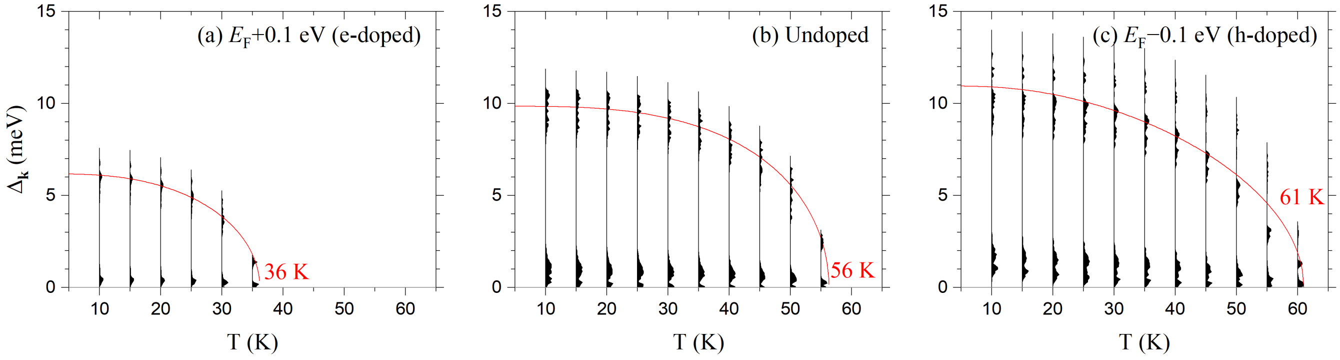


FIG. 12. Evolution of the anisotropic superconducting gap of AgBC as a function of temperature with (a) electron-doping (b) no doping and (c) hole-doping, achieved via rigid shifts of the Fermi level by ±0.1 eV.

# I. Note I - Energy units conversion

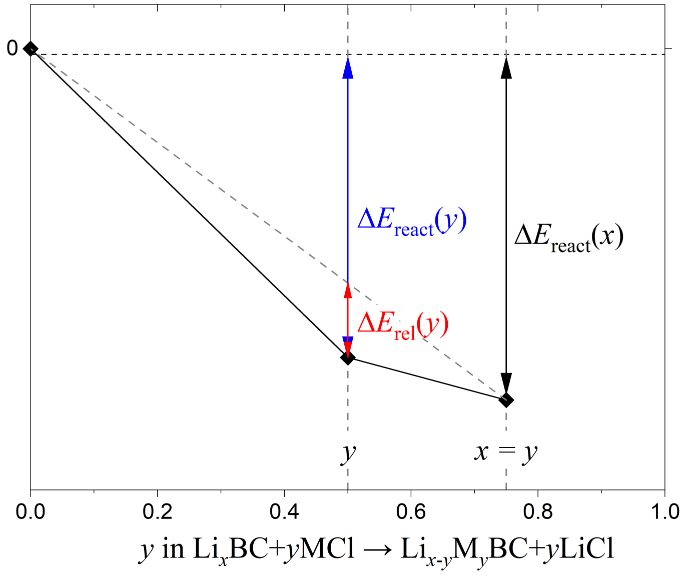


FIG. 13. Illustration of how relative energies $\Delta E_{\rm rel}(y)$ are found from reaction energies $\Delta E_{\rm react}(y)$ and $\Delta E_{\rm react}(x)$ in topochemical reactions with partial ion exchange between $Li_xBC$ precursors and $y$MCl salts.

In the case where non-stoichiometric $Li_xBC$ reacts with $y$MCl, the relative energy change, defined as the difference between the reaction energies at $y$ and $x$, can be expressed as:

$$\Delta E^{\rm mol}_{\rm rel}(y) = \Delta E^{\rm mol}_{\rm react}(y) - \frac{y}{x}\,\Delta E^{\rm mol}_{\rm react}(x).$$

Inserting the expression for $\Delta E_{\rm react}$ at each composition yields:

$$\begin{aligned}\Delta E^{\rm mol}_{\rm rel}(y) = {} & (2+x)\,{\rm Li}_{x-y}{\rm M}_y{\rm BC} + 2y\,{\rm LiCl} - (2+x)\,{\rm Li}_x{\rm BC} - 2y\,{\rm MCl} \\ & - \frac{y}{x}\Big[(2+x)\,{\rm M}_x{\rm BC} + 2x\,{\rm LiCl} - (2+x)\,{\rm Li}_x{\rm BC} - 2x\,{\rm MCl}\Big].\end{aligned}$$

After simplifying, the expression reduces to:

$$\Delta E^{\rm mol}_{\rm rel}(y) = (2+x)\left[{\rm Li}_{x-y}{\rm M}_y{\rm BC} - \frac{y}{x}\,{\rm M}_x{\rm BC} - \frac{x-y}{x}\,{\rm Li}_x{\rm BC}\right].$$

This result represents the distance to the convex hull for the $Li_{x-y}M_yBC$ phase relative to the $Li_xBC$ and $M_xBC$ endpoints, with the prefactor $(2+x)$ as a scaling constant. Consequently, the energy per atom (eV/atom) is related to the reaction energy per mole (kJ/mol) by:

$$\Delta E^{\rm atom}_{\rm rel}(y) = \frac{\Delta E^{\rm mol}_{\rm rel}(y)}{96.485\times(2+x)}.$$

## II. Note II - Approximation of the configurational free energy in $Li_{1-y}M_yBC$ (M = Cu or Ag)

We estimate the upper bound of the configurational entropy contribution for random Li-M-BC alloys using the standard assumption that all possible arrangements of Li and Cu on the metal sublattice are equiprobable [1]. Let $N$ denote the total number of atoms, and let $(1-y)$ and $y$ represent the fractions of Li and Cu atoms occupying the $M = N/3$ metal sites, respectively. If $n = yN/3$ is the number of Cu atoms replacing Li, the configurational multiplicity $\omega$ can be expressed as follows:

$$\omega = \binom{M}{M-n} = \frac{M!}{(M-n)!\,n!}.$$

Using Stirling's approximation, $\ln y! \approx y \ln y - y$, we write:

$$\ln \omega = n \ln\left(\frac{M}{n}\right) + (M-n)\ln\left(\frac{M}{M-n}\right).$$

Since $y = n/M$ and $1 - y = (M-n)/M$,

$$\ln \omega = -\frac{yN}{3}\ln y - \frac{(1-y)N}{3}\ln(1-y),$$
$$S_{\text{conf}}^{\text{total}} = k_B \ln \omega = -k_B \frac{N}{3}\left[y \ln y + (1-y)\ln(1-y)\right].$$

To obtain the configurational entropy per atom, we divide the total value by $N$:

$$S_{\text{conf}} = \frac{S_{\text{conf}}^{\text{total}}}{N} = -\frac{k_B}{3}\left[y \ln y + (1-y)\ln(1-y)\right],$$
$$F_{\text{conf}} = -TS_{\text{conf}} = \frac{k_B T}{3}\left[y \ln y + (1-y)\ln(1-y)\right].$$

For instance, at $y = 0.5$ and $T = 600\,\text{K}$, the configurational free energy is $F_{\text{conf}} = -0.012\,\text{eV/atom}$ ($-3.5\,\text{kJ/mol}$).

An additional configurational entropy contribution may appear in topochemical reactions if the exchanged ion forms a solid solution in the salt as well, such as $Li_xAg_{1-x}Cl$. Since the resulting fraction $x$ depends on the amount of the unreacted salt, the free energy change is subject to the choice of experimental conditions.

TABLE II. Structures used in topochemical reactions.

| Structure | Space group–Pearson symbol | Source |
|---|---|---|
| Li | 225–cF4 | mp–51 |
| Be | 194–hP2 | mp–87 |
| Na | 194–hP2 | mp–10172 |
| Mg | 194–hP2 | mp–153 |
| Cu | 225–cF4 | mp–30 |
| Zn | 194–hP2 | mp–79 |
| Ag | 225–cF4 | mp–124 |
| LiI | 225–cF8 | mp–22899 |
| $BeI_2$ | 142–tI96 | mp–30140 |
| NaI | 225–cF8 | mp–23268 |
| $MgI_2$ | 164–hP3 | mp–23205 |
| CuI | 156–hP12 | mp–570136 |
| $ZnI_2$ | 142–tI96 | mp–27161 |
| AgI | 186–hP8 | mp–580941 |
| LiBr | 225–cF8 | mp–23259 |
| $BeBr_2$ | 72–oI12 | mp–30139 |
| NaBr | 225–cF8 | mp–22916 |
| $MgBr_2$ | 164–hP3 | mp–30034 |
| CuBr | 216–cF8 | mp–22913 |
| $ZnBr_2$ | 142–tI96 | mp–647579 |
| AgBr | 225–cF8 | mp–23231 |
| LiCl | 225–cF8 | mp–22905 |
| $BeCl_2$ | 142–tI96 | mp–570974 |
| NaCl | 225–cF8 | mp–22862 |
| $MgCl_2$ | 166–hR9 | mp–23210 |
| CuCl | 216–cF8 | mp–22914 |
| $ZnCl_2$ | 122–tI12 | mp–22909 |
| AgCl | 225–cF8 | mp–22922 |
| $LiNO_3$ | 167–hR30 | mp–8180 |
| $NaNO_3$ | 167–hR30 | mp–4531 |
| $Mg(NO_3)_2$ | 205–cP36 | mp–771046 |
| $Zn(NO_3)_2$ | 205–cP36 | mp–772617 |
| $AgNO_3$ | 161–hR30 | mp–552185 |
| $Na_2IrO_3$ | 12–mS24 | mp–754844 |
| $Cu_2IrO_3$ | 15–mS48 | Abramchuk *et. al*–2017 [3] |
| $LiGaO_2$ | 33–oP16 | mp–5854 |
| $NaGaO_2$ | 33–oP16 | mp–3338 |
| $CuGaO_2$ | 33–oP16 | mp–1105229 |
| $AgGaO_2$ | 33–oP16 | mp–1105293 |
| LiBC | 194–hP6 | mp–9244 |
| $BeB_2C_2$ | 59–oP20 | mp–569299 |
| $MgB_2C_2$ | 64–oS80 | mp–3582 |

TABLE III. Settings used in the calculations of electronic, vibrational, and superconducting properties of Li-Cu-BC or Li-Ag-BC phases performed with QUANTUM ESPRESSO.

| Structure name | Pearson symbol | **k**-mesh | **q**-mesh |
|---|---|---|---|
| CuBC | mP6 | 30×30×8 | 4×4×2 |
| $Cu_{2/3}BC$ | hP16 | 18×18×8 | 6×6×3 |
| $Cu_{5/8}BC$ | hP21 | 18×18×8 | 6×6×3 |
| $Ag_{1/2}BC$ | oP10 | 18×18×12 | 4×4×3 |
| $Li_{1/6}Cu_{2/3}BC$ | hP17 | 18×18×8 | 6×6×3 |
| $Li_{1/2}Cu_{1/6}BC$ | hP16 | 18×18×8 | 6×6×3 |
| $Li_{1/2}Ag_{1/4}BC$ | hP22 | 18×18×8 | 6×6×3 |
| $Li_{1/4}Ag_{1/2}BC$ | oI22 | 30×18×2 | 6×3×2 |

Listing 1. CIF file for oI10-$Li_{1/2}BC$ containing the VASP optimized lattice constants and atomic positions.

```
_symmetry_Int_Tables_number 44
_cell_length_a 2.7244531594333852
_cell_length_b 7.0556539489437879
_cell_length_c 4.6112962278350889
_cell_angle_alpha 90.0000000000000000
_cell_angle_beta 90.0000000000000000
_cell_angle_gamma 90.0000000000000000
_symmetry_Int_Tables_number 44
_chemical_formula_sum
'Li B C '
loop_
_atom_site_label
_atom_site_type_symbol
_atom_site_site_symmetry_multiplicity
_atom_site_occupancy wyckoff
_atom_site_fract_x
_atom_site_fract_y
_atom_site_fract_z
Li1 Li 2 b 0.5000000000000000 0.0000000000000000 0.8205002134863698
B1 B 4 d 0.0000000000000000 0.7319152710952807 0.6883257945083586
C1 C 4 d 0.5000000000000000 0.7311169103590822 0.5243754051373727
#End
```

Listing 2. CIF file for oP21-$Li_{5/8}BC$ containing the VASP optimized lattice constants and atomic positions.

```
_symmetry_Int_Tables_number 25
_cell_length_a 2.7146362084270925
_cell_length_b 7.0615999001101279
_cell_length_c 9.1384658920936026
_cell_angle_alpha 90.0000000000000000
_cell_angle_beta 90.0000000000000000
_cell_angle_gamma 90.0000000000000000
_symmetry_Int_Tables_number 25
_chemical_formula_sum
'Li B C '
loop_
_atom_site_label
_atom_site_type_symbol
_atom_site_site_symmetry_multiplicity
_atom_site_occupancy wyckoff
_atom_site_fract_x
_atom_site_fract_y
_atom_site_fract_z
Li1 Li 1 a 0.0000000000000000 0.0000000000000000 0.2642718832612793
Li2 Li 1 b 0.0000000000000000 0.5000000000000000 0.7706289014430522
Li3 Li 1 c 0.5000000000000000 0.0000000000000000 0.5293259285147630
Li4 Li 1 d 0.5000000000000000 0.5000000000000000 0.4973519219425520
Li5 Li 1 b 0.0000000000000000 0.5000000000000000 0.2091260592680157
B1 B 2 h 0.5000000000000000 0.8227816652686458 0.8279882136061937
B2 B 2 h 0.5000000000000000 0.7461143625608933 0.3305370422687274
B3 B 2 g 0.0000000000000000 0.7372562661975890 0.5900115548818228
B4 B 2 g 0.0000000000000000 0.7959429578381925 0.0757409420852441
C1 C 2 h 0.5000000000000000 0.2345312813849527 0.1585665113052383
C2 C 2 h 0.5000000000000000 0.2643667512289111 0.6753390163231455
C3 C 2 g 0.0000000000000000 0.2561614399139010 0.4178258610141743
C4 C 2 g 0.0000000000000000 0.1152275367470387 0.9136385113006085
#End
```

Listing 3. CIF file for hP16-$Li_{2/3}BC$ containing the VASP optimized lattice constants and atomic positions.

```
_symmetry_Int_Tables_number 193
_cell_length_a 4.7043907314957547
_cell_length_b 4.7043907314957547
_cell_length_c 7.0677063573335817
_cell_angle_alpha 90.0000000000000000
_cell_angle_beta 90.0000000000000000
_cell_angle_gamma 120.0000000000000142
_symmetry_Int_Tables_number 193
_chemical_formula_sum
'Li B C '
loop_
_atom_site_label
_atom_site_type_symbol
_atom_site_site_symmetry_multiplicity
_atom_site_occupancy wyckoff
_atom_site_fract_x
_atom_site_fract_y
_atom_site_fract_z
Li1 Li 4 d 0.3333333333333333 0.6666666666666666 0.0000000000000000
B1 B 6 g 0.6705047023123636 0.6705047023123636 0.7500000000000000
C1 C 6 g 0.3368763332921496 0.0000000000000000 0.2500000000000000
#End
```

Listing 4. CIF file for oP22-$Li_{3/4}BC$ containing the VASP optimized lattice constants and atomic positions.

```
_symmetry_Int_Tables_number 55
_cell_length_a 7.1826361179194222
_cell_length_b 9.3753855918297475
_cell_length_c 2.7305648151975386
_cell_angle_alpha 90.0000000000000000
_cell_angle_beta 90.0000000000000000
_cell_angle_gamma 90.0000000000000000
_symmetry_Int_Tables_number 55
_chemical_formula_sum
'Li B C '
loop_
_atom_site_label
_atom_site_type_symbol
_atom_site_site_symmetry_multiplicity
_atom_site_occupancy wyckoff
_atom_site_fract_x
_atom_site_fract_y
_atom_site_fract_z
Li1 Li 2 c 0.5000000000000000 0.0000000000000000 0.0000000000000000
Li2 Li 4 h 0.0086012490286373 0.2265776417516029 0.5000000000000000
B1 B 4 g 0.7334409016578936 0.8288527887574426 0.0000000000000000
B2 B 4 h 0.2518678950089854 0.9226903391145680 0.5000000000000000
C1 C 4 h 0.7714359393289755 0.4106940742981678 0.5000000000000000
C2 C 4 g 0.2536761499217181 0.3389514682749687 0.0000000000000000
#End
```

Listing 5. CIF file for hP17-$Li_{5/6}BC$ containing the VASP optimized lattice constants and atomic positions.

```
_symmetry_Int_Tables_number 162
_cell_length_a 4.7301229712477788
_cell_length_b 4.7301229712477788
_cell_length_c 7.0543258471942218
_cell_angle_alpha 90.0000000000000000
```

```
_cell_angle_beta 90.0000000000000000
_cell_angle_gamma 120.0000000000000142
_symmetry_Int_Tables_number 162
_chemical_formula_sum
'Li B C '
loop_
_atom_site_label
_atom_site_type_symbol
_atom_site_site_symmetry_multiplicity
_atom_site_occupancy wyckoff
_atom_site_fract_x
_atom_site_fract_y
_atom_site_fract_z
Li1 Li 1 b 0.0000000000000000 0.0000000000000000 0.5000000000000000
Li2 Li 2 c 0.3333333333333333 0.6666666666666666 0.0000000000000000
Li3 Li 2 d 0.3333333333333333 0.6666666666666666 0.5000000000000000
B1 B 6 k 0.6684028392547275 0.6684028392547275 0.7495500302433904
C1 C 6 k 0.3349490690260606 0.0000000000000000 0.2531278106518320
#End
```

Listing 6. CIF file for hP23-$Li_{7/8}BC$ containing the VASP optimized lattice constants and atomic positions.

```
_symmetry_Int_Tables_number 164
_cell_length_a 5.4694797372616986
_cell_length_b 5.4694797372616977
_cell_length_c 7.0285011147524843
_cell_angle_alpha 90.0000000000000000
_cell_angle_beta 90.0000000000000000
_cell_angle_gamma 120.0000000000000142
_symmetry_Int_Tables_number 164
_chemical_formula_sum
'Li B C '
loop_
_atom_site_label
_atom_site_type_symbol
_atom_site_site_symmetry_multiplicity
_atom_site_occupancy wyckoff
_atom_site_fract_x
_atom_site_fract_y
_atom_site_fract_z
Li1 Li 3 e 0.5000000000000000 0.5000000000000000 0.0000000000000000
Li2 Li 3 f 0.5000000000000000 0.5000000000000000 0.5000000000000000
Li3 Li 1 a 0.0000000000000000 0.0000000000000000 0.0000000000000000
B1 B 6 i 0.8346598565800332 0.6693197131600664 0.7482368807851517
B2 B 2 d 0.3333333333333333 0.6666666666666666 0.7551608581006559
C1 C 6 i 0.8331081083354446 0.1668918916645554 0.2456916414987716
C2 C 2 d 0.3333333333333333 0.6666666666666666 0.2543727185638337
#End
```

Listing 7. CIF file for oP10-$Cu_{1/2}BC$ containing the VASP optimized lattice constants and atomic positions.

```
_symmetry_Int_Tables_number 26
_cell_length_a 3.4626468502450090
_cell_length_b 5.4759231875800829
_cell_length_c 4.6893393235631802
_cell_angle_alpha 90.0000000000000000
_cell_angle_beta 90.0000000000000000
_cell_angle_gamma 90.0000000000000000
_symmetry_Int_Tables_number 26
```

```
_chemical_formula_sum
'B C Cu '
loop_
_atom_site_label
_atom_site_type_symbol
_atom_site_site_symmetry_multiplicity
_atom_site_occupancy wyckoff
_atom_site_fract_x
_atom_site_fract_y
_atom_site_fract_z
B1 B 2 b 0.5000000000000000 0.8753230133589673 0.1381160908093640
B2 B 2 b 0.5000000000000000 0.6178401891083091 0.6307316968752804
C1 C 2 b 0.5000000000000000 0.3696801205568220 0.4650326904377675
C2 C 2 b 0.5000000000000000 0.8723668967992079 0.4767244900738434
Cu1 Cu 2 a 0.0000000000000000 0.1838841698273075 0.2893950318037524
#End
```

Listing 8. CIF file for hP21-$Cu_{5/8}BC$ containing the VASP optimized lattice constants and atomic positions.

```
_symmetry_Int_Tables_number 187
_cell_length_a 5.4506019817438371
_cell_length_b 5.4506019817438371
_cell_length_c 7.1860704332265604
_cell_angle_alpha 90.0000000000000000
_cell_angle_beta 90.0000000000000000
_cell_angle_gamma 120.0000000000000142
_symmetry_Int_Tables_number 187
_chemical_formula_sum
'B C Cu '
loop_
_atom_site_label
_atom_site_type_symbol
_atom_site_site_symmetry_multiplicity
_atom_site_occupancy wyckoff
_atom_site_fract_x
_atom_site_fract_y
_atom_site_fract_z
B1 B 2 h 0.3333333333333333 0.6666666666666666 0.7933819244910237
B2 B 6 n 0.8304223984482817 0.6608447968965633 0.7730055188120039
C1 C 2 i 0.6666666666666666 0.3333333333333333 0.7765457916407945
C2 C 6 n 0.6658522564118847 0.8329261282059424 0.7819938326386254
Cu1 Cu 3 k 0.6708775488403578 0.8354387744201789 0.5000000000000000
Cu2 Cu 1 f 0.6666666666666666 0.3333333333333333 0.5000000000000000
Cu3 Cu 1 a 0.0000000000000000 0.0000000000000000 0.0000000000000000
#End
```

Listing 9. CIF file for hP16-$Cu_{2/3}BC$ containing the VASP optimized lattice constants and atomic positions.

```
_symmetry_Int_Tables_number 189
_cell_length_a 4.7333929333515830
_cell_length_b 4.7333929333515821
_cell_length_c 7.2208810965200447
_cell_angle_alpha 90.0000000000000000
_cell_angle_beta 90.0000000000000000
_cell_angle_gamma 120.0000000000000142
_symmetry_Int_Tables_number 189
_chemical_formula_sum
'B C Cu '
loop_
```

```
_atom_site_label
_atom_site_type_symbol
_atom_site_site_symmetry_multiplicity
_atom_site_occupancy wyckoff
_atom_site_fract_x
_atom_site_fract_y
_atom_site_fract_z
B1 B 6 i 0.6634090109477675 0.6634090109477675 0.7750314803111406
C1 C 6 i 0.6679241033410251 0.0000000000000000 0.2215341581834210
Cu1 Cu 1 a 0.0000000000000000 0.0000000000000000 0.0000000000000000
Cu2 Cu 3 g 0.3197411978340756 0.3197411978340756 0.5000000000000000
#End
```

Listing 10. CIF file for oP22-$Cu_{3/4}$BC containing the VASP optimized lattice constants and atomic positions.

```
_symmetry_Int_Tables_number 26
_cell_length_a 7.3243560803813654
_cell_length_b 5.4441796871123858
_cell_length_c 4.7762240801071139
_cell_angle_alpha 90.0000000000000000
_cell_angle_beta 90.0000000000000000
_cell_angle_gamma 90.0000000000000000
_symmetry_Int_Tables_number 26
_chemical_formula_sum
'B C Cu '
loop_
_atom_site_label
_atom_site_type_symbol
_atom_site_site_symmetry_multiplicity
_atom_site_occupancy wyckoff
_atom_site_fract_x
_atom_site_fract_y
_atom_site_fract_z
B1 B 4 c 0.7605232290543269 0.8726066212561374 0.3409269763949718
B2 B 4 c 0.7775013751210579 0.6225803801467791 0.8457792435743777
C1 C 4 c 0.7761942228267696 0.3752468816223371 0.0148313865642939
C2 C 4 c 0.7722815352204691 0.8744388124138767 0.0111384310588729
Cu1 Cu 2 a 0.0000000000000000 0.8677467225446358 0.6161178176460453
Cu2 Cu 2 b 0.5000000000000000 0.8835581030697177 0.9968506693306729
Cu3 Cu 2 b 0.5000000000000000 0.6320681841772666 0.5233597882128507
#End
```

Listing 11. CIF file for mS34-$Cu_{5/6}$BC containing the VASP optimized lattice constants and atomic positions.

```
_symmetry_Int_Tables_number 8
_cell_length_a 4.7569063684550636
_cell_length_b 8.2508369865202074
_cell_length_c 7.7396996470704611
_cell_angle_alpha 90.0000000000000000
_cell_angle_beta 101.1750293941168479
_cell_angle_gamma 90.0000000000000000
_symmetry_Int_Tables_number 8
_chemical_formula_sum
'B C Cu '
loop_
_atom_site_label
_atom_site_type_symbol
_atom_site_site_symmetry_multiplicity
_atom_site_occupancy wyckoff
```

```
_atom_site_fract_x
_atom_site_fract_y
_atom_site_fract_z
B1 B 2 a 0.5702538265549455 0.0000000000000000 0.7640097116514539
B2 B 4 b 0.2852034942006256 0.1653167783329551 0.2420892946195113
B3 B 4 b 0.0657515932442392 0.1650745837512805 0.7633014576551640
B4 B 2 a 0.7928908276568993 0.0000000000000000 0.2463601790984338
C1 C 4 b 0.1240781926243824 0.3337773294072759 0.2408845230874677
C2 C 4 b 0.2348927998461918 0.3329361164466980 0.7669237022122988
C3 C 2 a 0.1232354376701505 0.0000000000000000 0.2500000000000000
C4 C 2 a 0.2385881139590418 0.0000000000000000 0.7742525453130005
Cu1 Cu 4 b 0.4618622954457426 0.1675566025104075 0.9837742907975258
Cu2 Cu 4 b 0.1523808497086525 0.3287438416237496 0.5019047152674022
Cu3 Cu 2 a 0.1763983872238480 0.0000000000000000 0.5108915105138646
#End
```

Listing 12. CIF file for mP23-$Cu_{7/8}BC$ containing the VASP optimized lattice constants and atomic positions.

```
_symmetry_Int_Tables_number 6
_cell_length_a 4.7795130044988516
_cell_length_b 5.4812036196884790
_cell_length_c 7.8094473794997903
_cell_angle_alpha 90.0000000000000000
_cell_angle_beta 102.4740072368924899
_cell_angle_gamma 90.0000000000000000
_symmetry_Int_Tables_number 6
_chemical_formula_sum
'B C Cu '
loop_
_atom_site_label
_atom_site_type_symbol
_atom_site_site_symmetry_multiplicity
_atom_site_occupancy wyckoff
_atom_site_fract_x
_atom_site_fract_y
_atom_site_fract_z
B1 B 2 c 0.7233436862663938 0.2463408833556814 0.0074458269013204
B2 B 2 c 0.6165519140209911 0.2474053441475025 0.4888336223330996
B3 B 1 a 0.2267171357932607 0.0000000000000000 0.0048304934631340
B4 B 1 a 0.1096531652578415 0.0000000000000000 0.4854073698472557
B5 B 1 b 0.2254432516866376 0.5000000000000000 0.0130136912544495
B6 B 1 b 0.1186003254706747 0.5000000000000000 0.5008687450498838
C1 C 1 a 0.5518967906477987 0.0000000000000000 0.9988597946664515
C2 C 1 a 0.4412852491804085 0.0000000000000000 0.4756486081049678
C3 C 1 b 0.5554668007556994 0.5000000000000000 0.0138226767360892
C4 C 1 b 0.4504830057654070 0.5000000000000000 0.4927954696446321
C5 C 2 c 0.0528978347772142 0.7510460635495837 0.0086019904564053
C6 C 2 c 0.9461737570970954 0.7502437884027472 0.4864866685526785
Cu1 Cu 1 b 0.5323593480594242 0.5000000000000000 0.7548045109577985
Cu2 Cu 1 a 0.4983753991313735 0.0000000000000000 0.7387720370065790
Cu3 Cu 1 b 0.7386165987199217 0.5000000000000000 0.2691790336640471
Cu4 Cu 2 c 0.0205442124485567 0.2519150938894630 0.7495835260372946
Cu5 Cu 2 c 0.2267952000652842 0.2469790586966721 0.2651943945343072
#End
```

Listing 13. CIF file for mP6-CuBC containing the VASP optimized lattice constants and atomic positions.

```
_symmetry_Int_Tables_number 6
_cell_length_a 2.7634828725337472
```

```
_cell_length_b 7.8678061763171643
_cell_length_c 2.7638833718080758
_cell_angle_alpha 90.0000000000000000
_cell_angle_beta 119.9810562886201950
_cell_angle_gamma 90.0000000000000000
_symmetry_Int_Tables_number 6
_chemical_formula_sum
'B C Cu '
loop_
_atom_site_label
_atom_site_type_symbol
_atom_site_site_symmetry_multiplicity
_atom_site_occupancy wyckoff
_atom_site_fract_x
_atom_site_fract_y
_atom_site_fract_z
B1 B 1 a 0.7055959395508064 0.0000000000000000 0.4412573449247458
B2 B 1 b 0.6657689751550740 0.5000000000000000 0.2333433108877092
C1 C 1 a 0.0416842249864933 0.0000000000000000 0.1137200887864216
C2 C 1 b 0.0013534300760307 0.5000000000000000 0.8973628799593610
Cu1 Cu 2 c 0.9829804317824555 0.2500000000000000 0.9904915210541847
#End
```

Listing 14. CIF file for oP10-$Ag_{1/2}BC$ containing the VASP optimized lattice constants and atomic positions.

```
_symmetry_Int_Tables_number 26
_cell_length_a 3.9922905664866963
_cell_length_b 5.4943987706202586
_cell_length_c 4.7066418142817943
_cell_angle_alpha 90.0000000000000000
_cell_angle_beta 90.0000000000000000
_cell_angle_gamma 90.0000000000000000
_symmetry_Int_Tables_number 26
_chemical_formula_sum
'B C Ag '
loop_
_atom_site_label
_atom_site_type_symbol
_atom_site_site_symmetry_multiplicity
_atom_site_occupancy wyckoff
_atom_site_fract_x
_atom_site_fract_y
_atom_site_fract_z
B1 B 2 a 0.0000000000000000 0.8800616101719504 0.3009772618562119
B2 B 2 a 0.0000000000000000 0.6252041397286171 0.7959631089358292
C1 C 2 a 0.0000000000000000 0.3729599360277976 0.9575318279257786
C2 C 2 a 0.0000000000000000 0.8716464522516194 0.9648140666665385
Ag1 Ag 2 b 0.5000000000000000 0.6968611294524958 0.1473804012822922
#End
```

Listing 15. CIF file for mS42-$Ag_{5/8}BC$ containing the VASP optimized lattice constants and atomic positions.

```
_symmetry_Int_Tables_number 5
_cell_length_a 9.4656421174734859
_cell_length_b 5.4695555297927170
_cell_length_c 9.0533633908839253
_cell_angle_alpha 90.0000000000000000
_cell_angle_beta 109.6612252355029113
_cell_angle_gamma 90.0000000000000000
```

```
_symmetry_Int_Tables_number 5
_chemical_formula_sum
'B C Ag '
loop_
_atom_site_label
_atom_site_type_symbol
_atom_site_site_symmetry_multiplicity
_atom_site_occupancy wyckoff
_atom_site_fract_x
_atom_site_fract_y
_atom_site_fract_z
B1 B 4 c 0.5836636243739062 0.7326238794352238 0.2465489818091546
B2 B 4 c 0.1670572703869085 0.9841902007936681 0.7473367613409660
B3 B 4 c 0.3342386254746754 0.9852341800204574 0.2438011093629124
B4 B 4 c 0.5843253925804475 0.2307445527534697 0.2495860210293199
C1 C 4 c 0.5820465138364905 0.7324313732029040 0.7486900941679847
C2 C 4 c 0.1666666666666667 0.9801073503057810 0.2440937048538028
C3 C 4 c 0.5835457170287003 0.2337007794904681 0.7536705366646407
C4 C 4 c 0.6676362743730353 0.9783640598654348 0.2569164894774372
Ag1 Ag 4 c 0.1585248604181643 0.8577962653843675 0.0017052576455070
Ag2 Ag 2 b 0.5000000000000000 0.3634881752786492 0.5000000000000000
Ag3 Ag 4 c 0.3333333333333333 0.8631634467652988 0.4933876410271446
#End
```

Listing 16. CIF file for oS32-$Ag_{2/3}BC$ containing the VASP optimized lattice constants and atomic positions.

```
_symmetry_Int_Tables_number 38
_cell_length_a 8.4189793557885135
_cell_length_b 2.7752525078909467
_cell_length_c 14.1855575421624334
_cell_angle_alpha 90.0000000000000000
_cell_angle_beta 90.0000000000000000
_cell_angle_gamma 90.0000000000000000
_symmetry_Int_Tables_number 38
_chemical_formula_sum
'B C Ag '
loop_
_atom_site_label
_atom_site_type_symbol
_atom_site_site_symmetry_multiplicity
_atom_site_occupancy wyckoff
_atom_site_fract_x
_atom_site_fract_y
_atom_site_fract_z
B1 B 4 c 0.7444175396495513 0.5000000000000000 0.2781701224840629
B2 B 4 c 0.7351812088922579 0.0000000000000000 0.4434304215963680
B3 B 4 c 0.7472074227315194 0.0000000000000000 0.1117785159986918
C1 C 4 c 0.7358922213942595 0.5000000000000000 0.4990307592811307
C2 C 4 c 0.7389163463388287 0.0000000000000000 0.3326411139060461
C3 C 4 c 0.7479129895881765 0.5000000000000000 0.1661715266549624
Ag1 Ag 2 a 0.0000000000000000 0.0000000000000000 0.3089020231891555
Ag2 Ag 2 b 0.5000000000000000 0.5000000000000000 0.0571871753421597
Ag3 Ag 2 a 0.0000000000000000 0.0000000000000000 0.0036508807947080
Ag4 Ag 2 b 0.5000000000000000 0.0000000000000000 0.2455927786092098
#End
```

Listing 17. CIF file for hR66-$Ag_{3/4}BC$ containing the VASP optimized lattice constants and atomic positions.

```
_symmetry_Int_Tables_number 155
```

```
_cell_length_a 5.5022583467109669
_cell_length_b 5.5022583467109669
_cell_length_c 25.6062614724646735
_cell_angle_alpha 90.0000000000000000
_cell_angle_beta 90.0000000000000000
_cell_angle_gamma 120.0000000000000142
_symmetry_Int_Tables_number 155
_chemical_formula_sum
'B C Ag '
loop_
_atom_site_label
_atom_site_type_symbol
_atom_site_site_symmetry_multiplicity
_atom_site_occupancy wyckoff
_atom_site_fract_x
_atom_site_fract_y
_atom_site_fract_z
B1 B 6 c 0.6666666666666666 0.3333333333333333 0.2500000000000000
B2 B 18 f 0.4958826894837641 0.4953290240564621 0.0833333333333333
C1 C 6 c 0.0000000000000000 0.0000000000000000 0.4175404972025451
C2 C 18 f 0.5033705592722661 0.5036997273324443 0.5833333333333334
Ag1 Ag 9 e 0.3333333333333333 0.9955436787812201 0.1666666666666667
Ag2 Ag 9 d 0.6486054498115661 0.6666666666666666 0.6666666666666666
#End
```

Listing 18. CIF file for mS34-$Ag_{5/6}BC$ containing the VASP optimized lattice constants and atomic positions.

```
_symmetry_Int_Tables_number 5
_cell_length_a 8.3289579243195657
_cell_length_b 4.8117874215663434
_cell_length_c 9.4491647129893312
_cell_angle_alpha 90.0000000000000000
_cell_angle_beta 109.4273955997960854
_cell_angle_gamma 90.0000000000000000
_symmetry_Int_Tables_number 5
_chemical_formula_sum
'B C Ag '
loop_
_atom_site_label
_atom_site_type_symbol
_atom_site_site_symmetry_multiplicity
_atom_site_occupancy wyckoff
_atom_site_fract_x
_atom_site_fract_y
_atom_site_fract_z
B1 B 4 c 0.5373651680848445 0.1269811638635858 0.7485730606687483
B2 B 4 c 0.3703691182027635 0.6239765992126607 0.7471935420316123
B3 B 4 c 0.2985516132293031 0.6228195422482965 0.2519421988367245
C1 C 4 c 0.0391963340898997 0.9567581094895847 0.7588270887460317
C2 C 4 c 0.6976224010127705 0.9552589934937101 0.7406316162750222
C3 C 4 c 0.1338337058896832 0.4561722111652695 0.2544918142785892
Ag1 Ag 4 c 0.1657771638556598 0.4645925032371343 0.4983151067430456
Ag2 Ag 4 c 0.8321905740099469 0.9641163813655833 0.9927779139356199
Ag3 Ag 2 a 0.0000000000000000 0.4652930886403656 0.0000000000000000
#End
```

Listing 19. CIF file for oP23-$Ag_{7/8}BC$ containing the VASP optimized lattice constants and atomic positions.

```
_symmetry_Int_Tables_number 25
```

```
_cell_length_a 2.7837665278316348
_cell_length_b 9.0636179026137942
_cell_length_c 9.5649556838191376
_cell_angle_alpha 90.0000000000000000
_cell_angle_beta 90.0000000000000000
_cell_angle_gamma 90.0000000000000000
_symmetry_Int_Tables_number 25
_chemical_formula_sum
'B C Ag '
loop_
_atom_site_label
_atom_site_type_symbol
_atom_site_site_symmetry_multiplicity
_atom_site_occupancy wyckoff
_atom_site_fract_x
_atom_site_fract_y
_atom_site_fract_z
B1 B 2 h 0.5000000000000000 0.7472181376260230 0.8333333333333334
B2 B 2 g 0.0000000000000000 0.7476598246158603 0.5821898412344296
B3 B 2 h 0.5000000000000000 0.7470080887506254 0.3315912869256242
B4 B 2 g 0.0000000000000000 0.7502848704302676 0.0800002324923612
C1 C 2 h 0.5000000000000000 0.7522016866737726 0.9999660050519185
C2 C 2 g 0.0000000000000000 0.7468674635441948 0.7503316269475686
C3 C 2 h 0.5000000000000000 0.7490113795730897 0.5000000000000000
C4 C 2 g 0.0000000000000000 0.7473944360255464 0.2494603589782290
Ag1 Ag 1 d 0.5000000000000000 0.5000000000000000 0.5042361249063635
Ag2 Ag 1 c 0.5000000000000000 0.0000000000000000 0.5002001461203108
Ag3 Ag 1 b 0.0000000000000000 0.5000000000000000 0.2272527613931812
Ag4 Ag 1 a 0.0000000000000000 0.0000000000000000 0.2488009184022805
Ag5 Ag 1 c 0.5000000000000000 0.0000000000000000 0.0000000000000000
Ag6 Ag 1 b 0.0000000000000000 0.5000000000000000 0.7809331397158514
Ag7 Ag 1 a 0.0000000000000000 0.0000000000000000 0.7515790922685175
#End
```

Listing 20. CIF file for hP3-AgBC containing the VASP optimized lattice constants and atomic positions.

```
_symmetry_Int_Tables_number 187
_cell_length_a 2.7916031552704030
_cell_length_b 2.7916031552704030
_cell_length_c 4.5798128995695819
_cell_angle_alpha 90.0000000000000000
_cell_angle_beta 90.0000000000000000
_cell_angle_gamma 120.0000000000000142
_symmetry_Int_Tables_number 187
_chemical_formula_sum
'B C Ag '
loop_
_atom_site_label
_atom_site_type_symbol
_atom_site_site_symmetry_multiplicity
_atom_site_occupancy wyckoff
_atom_site_fract_x
_atom_site_fract_y
_atom_site_fract_z
B1 B 1 a 0.0000000000000000 0.0000000000000000 0.0000000000000000
C1 C 1 e 0.6666666666666666 0.3333333333333333 0.0000000000000000
Ag1 Ag 1 f 0.6666666666666666 0.3333333333333333 0.5000000000000000
#End
```

Listing 21. CIF file for oS44-$Li_{1/8}Cu_{5/8}BC$ containing the VASP optimized lattice constants and atomic positions.

```
_symmetry_Int_Tables_number 38
_cell_length_a 7.2855146479744812
_cell_length_b 5.4819571066194879
_cell_length_c 9.4482073779015892
_cell_angle_alpha 90.0000000000000000
_cell_angle_beta 90.0000000000000000
_cell_angle_gamma 90.0000000000000000
_symmetry_Int_Tables_number 38
_chemical_formula_sum
'Li B C Cu '
loop_
_atom_site_label
_atom_site_type_symbol
_atom_site_site_symmetry_multiplicity
_atom_site_occupancy wyckoff
_atom_site_fract_x
_atom_site_fract_y
_atom_site_fract_z
Li1 Li 2 a 0.0000000000000000 0.0000000000000000 0.8447230287386343
B1 B 4 c 0.2178937384807580 0.0000000000000000 0.6648256830142480
B2 B 4 c 0.2259864669960905 0.0000000000000000 0.1637045159883026
B3 B 8 f 0.7638147434066510 0.7478762826366507 0.4179845021659836
C1 C 8 f 0.7779417160479041 0.7503649479656722 0.7487100615257640
C2 C 4 c 0.7722616356982879 0.0000000000000000 0.9991962721839946
C3 C 4 c 0.7762506243748156 0.0000000000000000 0.4991441721419190
Cu1 Cu 4 e 0.5000000000000000 0.2496379944641976 0.2500000000000000
Cu2 Cu 2 a 0.0000000000000000 0.0000000000000000 0.3412658282151244
Cu3 Cu 2 b 0.5000000000000000 0.0000000000000000 0.4949570976406015
Cu4 Cu 2 b 0.5000000000000000 0.0000000000000000 0.9984409913798542
#End
```

Listing 22. CIF file for hP17-$Li_{1/6}Cu_{2/3}BC$ containing the VASP optimized lattice constants and atomic positions.

```
_symmetry_Int_Tables_number 174
_cell_length_a 4.7513672531768041
_cell_length_b 4.7513672531768041
_cell_length_c 7.3317663029069919
_cell_angle_alpha 90.0000000000000000
_cell_angle_beta 90.0000000000000000
_cell_angle_gamma 120.0000000000000142
_symmetry_Int_Tables_number 174
_chemical_formula_sum
'Li B C Cu '
loop_
_atom_site_label
_atom_site_type_symbol
_atom_site_site_symmetry_multiplicity
_atom_site_occupancy wyckoff
_atom_site_fract_x
_atom_site_fract_y
_atom_site_fract_z
Li1 Li 1 f 0.6666666666666666 0.3333333333333333 0.5000000000000000
B1 B 6 l 0.3308654323635477 0.0002211794177059 0.7329738050572839
C1 C 6 l 0.3343927321369660 0.3344897322845854 0.7263626188310238
Cu1 Cu 1 d 0.3333333333333333 0.6666666666666666 0.5000000000000000
Cu2 Cu 3 j 0.0040130188556817 0.6566367030447475 0.0000000000000000
#End
```

Listing 23. CIF file for mP20-$Li_{1/4}Cu_{1/4}BC$ containing the VASP optimized lattice constants and atomic positions.

```
_symmetry_Int_Tables_number 13
_cell_length_a 6.9152656241889439
_cell_length_b 5.3861132562233376
_cell_length_c 4.7464496386721118
_cell_angle_alpha 90.0000000000000000
_cell_angle_beta 93.2208782670227407
_cell_angle_gamma 90.0000000000000000
_symmetry_Int_Tables_number 13
_chemical_formula_sum
'Li B C Cu '
loop_
_atom_site_label
_atom_site_type_symbol
_atom_site_site_symmetry_multiplicity
_atom_site_occupancy wyckoff
_atom_site_fract_x
_atom_site_fract_y
_atom_site_fract_z
Li1 Li 2 e 0.0000000000000000 0.1577879455997645 0.7500000000000000
B1 B 4 g 0.2487275342537397 0.8715172497660058 0.9287214255473473
B2 B 4 g 0.7332678158660848 0.6210219444119558 0.0647654201119790
C1 C 4 g 0.7362921169405720 0.3731106233463893 0.8911049545106462
C2 C 4 g 0.2509445393417036 0.1237769462277680 0.0993652659780430
Cu1 Cu 2 f 0.5000000000000000 0.1346342813335737 0.7500000000000000
#End
```

Listing 24. CIF file for oI22-$Li_{1/4}Cu_{1/2}BC$ containing the VASP optimized lattice constants and atomic positions.

```
_symmetry_Int_Tables_number 44
_cell_length_a 2.7423393238780402
_cell_length_b 14.8136948783493700
_cell_length_c 4.6916945196741873
_cell_angle_alpha 90.0000000000000000
_cell_angle_beta 90.0000000000000000
_cell_angle_gamma 90.0000000000000000
_symmetry_Int_Tables_number 44
_chemical_formula_sum
'Li B C Cu '
loop_
_atom_site_label
_atom_site_type_symbol
_atom_site_site_symmetry_multiplicity
_atom_site_occupancy wyckoff
_atom_site_fract_x
_atom_site_fract_y
_atom_site_fract_z
Li1 Li 2 a 0.5000000000000000 0.5000000000000000 0.6360132989490775
B1 B 4 d 0.0000000000000000 0.3794404536869435 0.7912068893046724
B2 B 4 d 0.0000000000000000 0.1128918359575589 0.7867572584198839
C1 C 4 d 0.0000000000000000 0.3893266896178920 0.4517921116589966
C2 C 4 d 0.0000000000000000 0.1181000014024161 0.4519188520342947
Cu1 Cu 4 d 0.5000000000000000 0.2466726805691570 0.9512498159885444
#End
```

Listing 25. CIF file for hP15-$Li_{1/3}Cu_{1/6}BC$ containing the VASP optimized lattice constants and atomic positions.

```
_symmetry_Int_Tables_number 149
_cell_length_a 4.7017859974395879
```

```
_cell_length_b 4.7017859974395879
_cell_length_c 6.9039067371354106
_cell_angle_alpha 90.0000000000000000
_cell_angle_beta 90.0000000000000000
_cell_angle_gamma 120.0000000000000142
_symmetry_Int_Tables_number 149
_chemical_formula_sum
'Li B C Cu '
loop_
_atom_site_label
_atom_site_type_symbol
_atom_site_site_symmetry_multiplicity
_atom_site_occupancy wyckoff
_atom_site_fract_x
_atom_site_fract_y
_atom_site_fract_z
Li1 Li 1 e 0.6666666666666666 0.3333333333333333 0.0000000000000000
Li2 Li 1 b 0.0000000000000000 0.0000000000000000 0.5000000000000000
B1 B 6 l 0.6628470513885062 0.6651558263626275 0.2468541376991529
C1 C 6 l 0.9980450768074041 0.6700169720868109 0.2440040329442017
Cu1 Cu 1 a 0.0000000000000000 0.0000000000000000 0.0000000000000000
#End
```

Listing 26. CIF file for hP16-$Li_{1/3}Cu_{1/3}BC$ containing the VASP optimized lattice constants and atomic positions.

```
_symmetry_Int_Tables_number 173
_cell_length_a 4.7314148298519285
_cell_length_b 4.7314148298519285
_cell_length_c 6.8776644176003794
_cell_angle_alpha 90.0000000000000000
_cell_angle_beta 90.0000000000000000
_cell_angle_gamma 120.0000000000000142
_symmetry_Int_Tables_number 173
_chemical_formula_sum
'Li B C Cu '
loop_
_atom_site_label
_atom_site_type_symbol
_atom_site_site_symmetry_multiplicity
_atom_site_occupancy wyckoff
_atom_site_fract_x
_atom_site_fract_y
_atom_site_fract_z
Li1 Li 2 b 0.3333333333333333 0.6666666666666666 0.2500000000000000
B1 B 6 c 0.6710288126234141 0.0000000000000000 0.0000000000000000
C1 C 6 c 0.3375885639655249 0.3363221405023087 0.5000000000000000
Cu1 Cu 2 b 0.3333333333333333 0.6666666666666666 0.7500000000000000
#End
```

Listing 27. CIF file for hP34-$Li_{1/3}Cu_{1/2}BC$ containing the VASP optimized lattice constants and atomic positions.

```
_symmetry_Int_Tables_number 193
_cell_length_a 4.7379849872072191
_cell_length_b 4.7379849872072191
_cell_length_c 14.7358738997424261
_cell_angle_alpha 90.0000000000000000
_cell_angle_beta 90.0000000000000000
_cell_angle_gamma 120.0000000000000142
_symmetry_Int_Tables_number 193
```

```
_chemical_formula_sum
'Li B C Cu '
loop_
_atom_site_label
_atom_site_type_symbol
_atom_site_site_symmetry_multiplicity
_atom_site_occupancy wyckoff
_atom_site_fract_x
_atom_site_fract_y
_atom_site_fract_z
Li1 Li 4 d 0.6666666666666666 0.3333333333333333 0.0000000000000000
B1 B 12 k 0.3309480361691263 0.0000000000000000 0.1173962386997877
C1 C 12 k 0.3345341892918806 0.3345341892918806 0.1141809034942118
Cu1 Cu 6 g 0.3403844840274831 0.3403844840274831 0.2500000000000000
#End
```

Listing 28. CIF file for mP21-$Li_{3/8}Cu_{1/4}BC$ containing the VASP optimized lattice constants and atomic positions.

```
_symmetry_Int_Tables_number 3
_cell_length_a 4.7092794301157950
_cell_length_b 5.4627830959700958
_cell_length_c 6.9098130170901451
_cell_angle_alpha 90.0000000000000000
_cell_angle_beta 90.3968493190237012
_cell_angle_gamma 90.0000000000000000
_symmetry_Int_Tables_number 3
_chemical_formula_sum
'Li B C Cu '
loop_
_atom_site_label
_atom_site_type_symbol
_atom_site_site_symmetry_multiplicity
_atom_site_occupancy wyckoff
_atom_site_fract_x
_atom_site_fract_y
_atom_site_fract_z
Li1 Li 1 d 0.5000000000000000 0.7608202778880832 0.5000000000000000
Li2 Li 1 a 0.0000000000000000 0.5095225305515997 0.0000000000000000
Li3 Li 1 d 0.5000000000000000 0.2470657603239754 0.5000000000000000
B1 B 2 e 0.6728873666579486 0.9984453537224539 0.2553532118141324
B2 B 2 e 0.8333333333333334 0.2484139428488938 0.7521484053122938
B3 B 2 e 0.6663228967018122 0.5021820733198655 0.2486314662845366
B4 B 2 e 0.8315773844609468 0.7557654204542333 0.7552321884777972
C1 C 2 e 0.6718018796344257 0.5017440603219335 0.7464321195657680
C2 C 2 e 0.8362195127640961 0.7484065056514891 0.2524639775302516
C3 C 2 e 0.6617952288792753 0.0028588609339360 0.7464532702970837
C4 C 2 e 0.8303883547022167 0.2516329352887856 0.2457350781099502
Cu1 Cu 1 b 0.0000000000000000 0.5267320082244727 0.5000000000000000
Cu2 Cu 1 c 0.5000000000000000 0.1869611179286774 0.0000000000000000
#End
```

Listing 29. CIF file for oP46-$Li_{3/8}Cu_{1/2}BC$ containing the VASP optimized lattice constants and atomic positions.

```
_symmetry_Int_Tables_number 51
_cell_length_a 14.6910248632536931
_cell_length_b 5.4759508764569844
_cell_length_c 4.7506810634032961
_cell_angle_alpha 90.0000000000000000
_cell_angle_beta 90.0000000000000000
```

```
_cell_angle_gamma 90.0000000000000000
_symmetry_Int_Tables_number 51
_chemical_formula_sum
'Li B C Cu '
loop_
_atom_site_label
_atom_site_type_symbol
_atom_site_site_symmetry_multiplicity
_atom_site_occupancy wyckoff
_atom_site_fract_x
_atom_site_fract_y
_atom_site_fract_z
Li1 Li 4 g 0.5000000000000000 0.7580336645075745 0.0000000000000000
Li2 Li 2 d 0.5000000000000000 0.5000000000000000 0.5000000000000000
B1 B 8 l 0.3832702686152056 0.2475908489256645 0.3352505923713217
B2 B 4 i 0.6177164165469700 0.0000000000000000 0.1690978677007962
B3 B 4 j 0.1188408402564928 0.5000000000000000 0.8336217450512717
C1 C 4 j 0.1129441272380700 0.5000000000000000 0.1677345675592746
C2 C 8 l 0.3858340661022504 0.7500000000000000 0.6662550515129219
C3 C 4 i 0.6140426560636959 0.0000000000000000 0.8352206399598849
Cu1 Cu 4 k 0.7500000000000000 0.7468212857301082 0.3312490210617697
Cu2 Cu 2 f 0.7500000000000000 0.5000000000000000 0.8279449707204656
Cu3 Cu 2 e 0.2500000000000000 0.0000000000000000 0.1602931717141965
#End
```

Listing 30. CIF file for mP21-$Li_{1/2}Cu_{1/8}BC$ containing the VASP optimized lattice constants and atomic positions.

```
_symmetry_Int_Tables_number 3
_cell_length_a 4.7314166437458853
_cell_length_b 5.4124957447567548
_cell_length_c 7.0184690044444391
_cell_angle_alpha 90.0000000000000000
_cell_angle_beta 90.9630162076578017
_cell_angle_gamma 90.0000000000000000
_symmetry_Int_Tables_number 3
_chemical_formula_sum
'Li B C Cu '
loop_
_atom_site_label
_atom_site_type_symbol
_atom_site_site_symmetry_multiplicity
_atom_site_occupancy wyckoff
_atom_site_fract_x
_atom_site_fract_y
_atom_site_fract_z
Li1 Li 1 c 0.5000000000000000 0.7563894283119728 0.0000000000000000
Li2 Li 1 b 0.0000000000000000 0.5163895069839309 0.5000000000000000
Li3 Li 1 d 0.5000000000000000 0.2176941740558284 0.5000000000000000
Li4 Li 1 c 0.5000000000000000 0.2466013911722757 0.0000000000000000
B1 B 2 e 0.6723590715463307 0.9987614508156278 0.7604823790182772
B2 B 2 e 0.8311301620007066 0.2462405087746080 0.2469855226928068
B3 B 2 e 0.6680899419832790 0.5016852909754533 0.7500000000000000
B4 B 2 e 0.8283523412838190 0.7553365199063343 0.2483209256425351
C1 C 2 e 0.6632981552449747 0.5005247306037602 0.2488611371715796
C2 C 2 e 0.8427961207114484 0.7486346083900096 0.7584635059160642
C3 C 2 e 0.6531236256312977 0.0012825083134858 0.2411036875158498
C4 C 2 e 0.8398634503369286 0.2517555997513686 0.7542791841575572
Cu1 Cu 1 a 0.0000000000000000 0.5044830644146673 0.0000000000000000
#End
```

Listing 31. CIF file for hP16-$Li_{1/2}Cu_{1/6}BC$ containing the VASP optimized lattice constants and atomic positions.

```
_symmetry_Int_Tables_number 149
_cell_length_a 4.7216563865824615
_cell_length_b 4.7216563865824615
_cell_length_c 6.9416770552157905
_cell_angle_alpha 90.0000000000000000
_cell_angle_beta 90.000000000000000
_cell_angle_gamma 120.0000000000000142
_symmetry_Int_Tables_number 149
_chemical_formula_sum
'Li B C Cu '
loop_
_atom_site_label
_atom_site_type_symbol
_atom_site_site_symmetry_multiplicity
_atom_site_occupancy wyckoff
_atom_site_fract_x
_atom_site_fract_y
_atom_site_fract_z
Li1 Li 1 b 0.0000000000000000 0.0000000000000000 0.5000000000000000
Li2 Li 1 c 0.3333333333333333 0.6666666666666666 0.0000000000000000
Li3 Li 1 d 0.3333333333333333 0.6666666666666666 0.5000000000000000
B1 B 6 l 0.3369949623412676 0.3327418879075366 0.2471577811065022
C1 C 6 l 0.3289382623699615 0.3319406042149451 0.7523575045974455
Cu1 Cu 1 a 0.0000000000000000 0.0000000000000000 0.0000000000000000
#End
```

Listing 32. CIF file for hP12-$Li_{1/2}Cu_{1/2}BC$ containing the VASP optimized lattice constants and atomic positions.

```
_symmetry_Int_Tables_number 194
_cell_length_a 2.7557614068396825
_cell_length_b 2.7557614068396825
_cell_length_c 14.5614997902876180
_cell_angle_alpha 90.0000000000000000
_cell_angle_beta 90.000000000000000
_cell_angle_gamma 120.0000000000000142
_symmetry_Int_Tables_number 194
_chemical_formula_sum
'Li B C Cu '
loop_
_atom_site_label
_atom_site_type_symbol
_atom_site_site_symmetry_multiplicity
_atom_site_occupancy wyckoff
_atom_site_fract_x
_atom_site_fract_y
_atom_site_fract_z
Li1 Li 2 a 0.0000000000000000 0.0000000000000000 0.0000000000000000
B1 B 4 f 0.3333333333333333 0.6666666666666666 0.1180809023683886
C1 C 4 f 0.6666666666666666 0.3333333333333333 0.1127363030225145
Cu1 Cu 2 d 0.6666666666666666 0.3333333333333333 0.2500000000000000
#End
```

Listing 33. CIF file for hP9-$Li_{2/3}Cu_{1/3}BC$ containing the VASP optimized lattice constants and atomic positions.

```
_symmetry_Int_Tables_number 187
```

```
_cell_length_a 2.7530708446108152
_cell_length_b 2.7530708446108152
_cell_length_c 10.7615665055206655
_cell_angle_alpha 90.0000000000000000
_cell_angle_beta 90.0000000000000000
_cell_angle_gamma 120.0000000000000142
_symmetry_Int_Tables_number 187
_chemical_formula_sum
'Li B C Cu '
loop_
_atom_site_label
_atom_site_type_symbol
_atom_site_site_symmetry_multiplicity
_atom_site_occupancy wyckoff
_atom_site_fract_x
_atom_site_fract_y
_atom_site_fract_z
Li1 Li 2 g 0.0000000000000000 0.0000000000000000 0.8391925582242618
B1 B 1 e 0.6666666666666666 0.3333333333333333 0.0000000000000000
B2 B 2 h 0.3333333333333333 0.6666666666666666 0.3213426209482579
C1 C 1 c 0.3333333333333333 0.6666666666666666 0.0000000000000000
C2 C 2 i 0.6666666666666666 0.3333333333333333 0.3140484997665451
Cu1 Cu 1 f 0.6666666666666666 0.3333333333333333 0.5000000000000000
#End
```

Listing 34. CIF file for mP21-$Li_{1/8}Ag_{1/2}BC$ containing the VASP optimized lattice constants and atomic positions.

```
_symmetry_Int_Tables_number 10
_cell_length_a 4.7771146474112252
_cell_length_b 2.7607363318879039
_cell_length_c 14.8421217518755348
_cell_angle_alpha 90.0000000000000000
_cell_angle_beta 90.3023625844492130
_cell_angle_gamma 90.0000000000000000
_symmetry_Int_Tables_number 10
_chemical_formula_sum
'Li B C Ag '
loop_
_atom_site_label
_atom_site_type_symbol
_atom_site_site_symmetry_multiplicity
_atom_site_occupancy wyckoff
_atom_site_fract_x
_atom_site_fract_y
_atom_site_fract_z
Li1 Li 1 e 0.5000000000000000 0.5000000000000000 0.0000000000000000
B1 B 2 n 0.8293589804647520 0.5000000000000000 0.5797994805246554
B2 B 2 m 0.6704842153879662 0.0000000000000000 0.4205412937256762
B3 B 2 n 0.8451918301862760 0.5000000000000000 0.8899364666250251
B4 B 2 m 0.6601872677256085 0.0000000000000000 0.1157522949951291
C1 C 2 m 0.6628064397246988 0.0000000000000000 0.5843382217519084
C2 C 2 m 0.6762922562548972 0.0000000000000000 0.8904279729584101
C3 C 2 n 0.1628405115554535 0.5000000000000000 0.5819049447126452
C4 C 2 n 0.1758773284085851 0.5000000000000000 0.8854895338133366
Ag1 Ag 2 n 0.1702091067761590 0.5000000000000000 0.7333304565230284
Ag2 Ag 2 m 0.3301732350903395 0.0000000000000000 0.2630471385726246
#End
```

Listing 35. CIF file for hP32-$Li_{1/6}Ag_{1/2}BC$ containing the VASP optimized lattice constants and atomic positions.

```
_symmetry_Int_Tables_number 162
_cell_length_a 4.7846648790633690
_cell_length_b 4.7846648790633690
_cell_length_c 14.8894714074382239
_cell_angle_alpha 90.0000000000000000
_cell_angle_beta 90.0000000000000000
_cell_angle_gamma 120.0000000000000142
_symmetry_Int_Tables_number 162
_chemical_formula_sum
'Li B C Ag '
loop_
_atom_site_label
_atom_site_type_symbol
_atom_site_site_symmetry_multiplicity
_atom_site_occupancy wyckoff
_atom_site_fract_x
_atom_site_fract_y
_atom_site_fract_z
Li1 Li 2 d 0.3333333333333333 0.6666666666666666 0.5000000000000000
B1 B 6 k 0.6692601636758280 0.0000000000000000 0.3854044457127326
B2 B 6 k 0.3333333333333333 0.3333333333333333 0.0803413661891182
C1 C 6 k 0.3333333333333333 0.0000000000000000 0.0837883637269500
C2 C 6 k 0.3345214688582037 0.0000000000000000 0.3873186300731732
Ag1 Ag 6 k 0.0000000000000000 0.3341054349170158 0.2347860209097685
#End
```

Listing 36. CIF file for mP20-$Li_{1/4}Ag_{1/4}BC$ containing the VASP optimized lattice constants and atomic positions.

```
_symmetry_Int_Tables_number 13
_cell_length_a 7.4529060145745101
_cell_length_b 5.4319724123989088
_cell_length_c 4.7243281755142830
_cell_angle_alpha 90.0000000000000000
_cell_angle_beta 91.2991486828092320
_cell_angle_gamma 90.0000000000000000
_symmetry_Int_Tables_number 13
_chemical_formula_sum
'Li B C Ag '
loop_
_atom_site_label
_atom_site_type_symbol
_atom_site_site_symmetry_multiplicity
_atom_site_occupancy wyckoff
_atom_site_fract_x
_atom_site_fract_y
_atom_site_fract_z
Li1 Li 2 e 0.0000000000000000 0.1481408382929961 0.2500000000000000
B1 B 4 g 0.2318671408190345 0.8724436988859059 0.4234805930398965
B2 B 4 g 0.7628105207311734 0.6213690742620395 0.5719974995791075
C1 C 4 g 0.7638064025025371 0.3736939395248347 0.4026454402032457
C2 C 4 g 0.2295078177973280 0.1251314389659767 0.5903923969032321
Ag1 Ag 2 f 0.5000000000000000 0.1711153136804924 0.2500000000000000
#End
```

Listing 37. CIF file for oI22-$Li_{1/4}Ag_{1/2}BC$ containing the VASP optimized lattice constants and atomic positions.

```
_symmetry_Int_Tables_number 44
_cell_length_a 2.7705319697465072
```

```
_cell_length_b 15.6278572612713074
_cell_length_c 4.7769435779262777
_cell_angle_alpha 90.0000000000000000
_cell_angle_beta 90.0000000000000000
_cell_angle_gamma 90.0000000000000000
_symmetry_Int_Tables_number 44
_chemical_formula_sum
'Li B C Ag '
loop_
_atom_site_label
_atom_site_type_symbol
_atom_site_site_symmetry_multiplicity
_atom_site_occupancy wyckoff
_atom_site_fract_x
_atom_site_fract_y
_atom_site_fract_z
Li1 Li 2 b 0.5000000000000000 0.0000000000000000 0.6321799074976614
B1 B 4 d 0.0000000000000000 0.8894924726470256 0.7895977134174728
B2 B 4 d 0.0000000000000000 0.6042658763536708 0.7842360434334621
C1 C 4 d 0.0000000000000000 0.8971733143279095 0.4518966356863222
C2 C 4 d 0.0000000000000000 0.6097788109666329 0.4522042382740201
Ag1 Ag 4 d 0.5000000000000000 0.7466990323514503 0.9569069923208222
#End
```

Listing 38. CIF file for hP34-$Li_{1/3}Ag_{1/2}BC$ containing the VASP optimized lattice constants and atomic positions.

```
_symmetry_Int_Tables_number 193
_cell_length_a 4.8019286731992494
_cell_length_b 4.8019286731992494
_cell_length_c 15.6184124509975248
_cell_angle_alpha 90.0000000000000000
_cell_angle_beta 90.0000000000000000
_cell_angle_gamma 120.0000000000000142
_symmetry_Int_Tables_number 193
_chemical_formula_sum
'Li B C Ag '
loop_
_atom_site_label
_atom_site_type_symbol
_atom_site_site_symmetry_multiplicity
_atom_site_occupancy wyckoff
_atom_site_fract_x
_atom_site_fract_y
_atom_site_fract_z
Li1 Li 4 d 0.3333333333333333 0.6666666666666666 0.0000000000000000
B1 B 12 k 0.3305815198127019 0.3305815198127019 0.1085811469255254
C1 C 12 k 0.3344426610924789 0.0000000000000000 0.1067873861931809
Ag1 Ag 6 g 0.3351293247314804 0.3351293247314804 0.7500000000000000
#End
```

Listing 39. CIF file for oP46-$Li_{3/8}Ag_{1/2}BC$ containing the VASP optimized lattice constants and atomic positions.

```
_symmetry_Int_Tables_number 51
_cell_length_a 15.5960794799639260
_cell_length_b 5.5549959723712039
_cell_length_c 4.8084052513913855
_cell_angle_alpha 90.0000000000000000
_cell_angle_beta 90.0000000000000000
_cell_angle_gamma 90.0000000000000000
```

```
_symmetry_Int_Tables_number 51
_chemical_formula_sum
'Li B C Ag '
loop_
_atom_site_label
_atom_site_type_symbol
_atom_site_site_symmetry_multiplicity
_atom_site_occupancy wyckoff
_atom_site_fract_x
_atom_site_fract_y
_atom_site_fract_z
Li1 Li 4 h 0.5000000000000000 0.7566308547524652 0.5000000000000000
Li2 Li 2 b 0.5000000000000000 0.5000000000000000 0.0000000000000000
B1 B 8 l 0.3918137745651090 0.2474058761047481 0.8352375232992379
B2 B 4 i 0.6091361713795359 0.0000000000000000 0.6695986853278957
B3 B 4 j 0.1100264241301421 0.5000000000000000 0.3333333333333333
C1 C 4 j 0.1056157402701421 0.5000000000000000 0.6681946117487627
C2 C 8 l 0.3929633343096745 0.7500000000000000 0.1666666666666667
C3 C 4 i 0.6068971771879671 0.0000000000000000 0.3345008126403275
Ag1 Ag 4 k 0.7500000000000000 0.7492954836652288 0.8320774025256461
Ag2 Ag 2 f 0.7500000000000000 0.5000000000000000 0.3305909414324326
Ag3 Ag 2 e 0.2500000000000000 0.0000000000000000 0.6654749648237739
#End
```

Listing 40. CIF file for hP12-$Li_{1/2}Ag_{1/2}BC$ containing the VASP optimized lattice constants and atomic positions.

```
_symmetry_Int_Tables_number 194
_cell_length_a 2.7895089222478768
_cell_length_b 2.7895089222478768
_cell_length_c 15.5523685936558866
_cell_angle_alpha 90.0000000000000000
_cell_angle_beta 90.0000000000000000
_cell_angle_gamma 120.0000000000000142
_symmetry_Int_Tables_number 194
_chemical_formula_sum
'Li B C Ag '
loop_
_atom_site_label
_atom_site_type_symbol
_atom_site_site_symmetry_multiplicity
_atom_site_occupancy wyckoff
_atom_site_fract_x
_atom_site_fract_y
_atom_site_fract_z
Li1 Li 2 a 0.0000000000000000 0.0000000000000000 0.5000000000000000
B1 B 4 f 0.6666666666666666 0.3333333333333333 0.3901576741799203
C1 C 4 f 0.3333333333333333 0.6666666666666666 0.3939716927467318
Ag1 Ag 2 c 0.3333333333333333 0.6666666666666666 0.2500000000000000
#End
```

[1] C. R. Tomassetti, D. Gochitashvili, C. Renskers, E. R. Margine, and A. N. Kolmogorov, First-principles design of ambient-pressure $Mg_xB_2C_2$ and $Na_xBC$ superconductors, Physical Review Materials **8**, 114801 (2024).
[2] I. Suzuki, M. Kita, and T. Omata, Designing Topotactic Ion-Exchange Reactions in Solid-State Oxides Through First-Principles Calculations, Chemistry of Materials **36**, 4196 (2024).
[3] M. Abramchuk, C. Ozsoy-Keskinbora, J. W. Krizan, K. R. Metz, D. C. Bell, and F. Tafti, $Cu_2IrO_3$: A New Magnetically Frustrated Honeycomb Iridate, Journal of the American Chemical Society **139**, 15371 (2017).
